# Supplementary material for: Machine learning applications using diffusion tensor imaging of human brain: A PubMed literature review
Source: arXiv:2012.10517 ancillary file (2020-12-18)
Supplement: Supplementary file 1 [file Supplementary_DTI_paper_v5.pdf]

# Supplementary File for “Machine learning applications using Diffusion Tensor Imaging of human brain: A PubMed Literature Review”

Ashirbani Saha<sup>1</sup>, Pantea Fadaiefard<sup>1</sup>, Jessica Rabski<sup>1</sup>, Alireza Sadeghian<sup>2</sup>, and Michael D. Cusimano<sup>1,3</sup>

<sup>1</sup>Injury Prevention Research Office, St. Michael’s Hospital, Toronto, ON, Canada

<sup>2</sup>Department of Computer Science, Ryerson University, Canada,

<sup>3</sup> Division of Neurosurgery, Department of Surgery, University of Toronto, Toronto, ON, Canada

## Search Criteria:

Three search strings were used using ‘human’ as filter for date range 01-01-2010 to 31-12-2019 in April 2020

(a) diffusion tensor imaging machine learning

(b) diffusion tensor imaging deep learning

(c) ("brain"[MeSH Terms] OR "brain"[All Fields]) AND (("diffusion magnetic resonance imaging"[MeSH Terms] OR "diffusion magnetic resonance imaging"[All Fields]) OR ("Diffusion Tensor Imaging"[MeSH Terms] OR "diffusion tensor imaging"[All Fields]) OR Tractography[All Fields] OR ("connectome"[MeSH Terms] OR "connectome"[All Fields]))AND (("machine learning"[MeSH Terms] OR "machine learning"[All Fields]) OR ("deep learning"[MeSH Terms] OR "deep learning"[All Fields]) OR ("artificial intelligence"[MeSH Terms] OR "artificial intelligence"[All Fields]))

## Details of the reviewed studied:

**Table 1 Details of the studies that focused on healthy cohorts**

| Serial Number | First Author, Publication Venue, Year, Reference | Unmet Need                                                                                                          | ML Task Performed                                                                                                                                         | Reference Standard                                                                             | Role of DTI                                                                        | Machine Learning models used               | Accomplishments and Limitations (including what authors stated)                                                                                                                                                                                                  |
|---------------|--------------------------------------------------|---------------------------------------------------------------------------------------------------------------------|-----------------------------------------------------------------------------------------------------------------------------------------------------------|------------------------------------------------------------------------------------------------|------------------------------------------------------------------------------------|--------------------------------------------|------------------------------------------------------------------------------------------------------------------------------------------------------------------------------------------------------------------------------------------------------------------|
| 1             | A. Ciritsis, NMR in Biomedicine, 2018 [1]        | Automated pixel-wise cerebral tissue segmentation using diffusion imaging acquired at several b-values (mostly low) | Automatic segmentation of brain tissue in healthy human subjects (dataset of 8)                                                                           | Software-generated (SPM12 generated tissue classification probability maps after thresholding) | To estimate trace and extract FA                                                   | SVM (one-versus-all classification scheme) | A: Tissue segmentation was performed with high accuracy (82.1% in the validation dataset). L: Comparison to a standard tool as reference, noise effect on highly resolved DWI with high b-values and by the long acquisition times; used healthy volunteers only |
| 2             | N. S. Gorbach, NeuroImage, 2018 [2]              | To assess the quality of the parcellation within an individual brain is apparent in brain mapping.                  | Validation method to identify a pipeline of algorithms that is robust to noise in diffusion MRI for connectivity-based cortex parcellation (dataset of 3) | Anatomical interpretation of labels based on prior works                                       | To estimate of diffusion tensor information that guides the tractography performed | Validation of several algorithms           | A: Identification of a pipeline of algorithms that are more noise tolerant and can extract more parameters (code available) L: Small set                                                                                                                         |
| 3             | S. Genon, NeuroImage, 2018 [3]                   | To provide the first robust modular map of the left dorsal                                                          | Parcellation of sub-regions of left- PMd in healthy adults for                                                                                            | Cytotechnic architecture behavioral mapping                                                    | To validate structural connectivity used in                                        | K-means                                    | A: A parcellation of the left premotor cortex into 5 robust modules was                                                                                                                                                                                          |

|   |                                                                |                                                                                                                             |                                                                                                                         |                                                                        |                                                                                                         |                                                                                                                                                               |                                                                                                                                                                                                                                                                                                                                                                                                          |
|---|----------------------------------------------------------------|-----------------------------------------------------------------------------------------------------------------------------|-------------------------------------------------------------------------------------------------------------------------|------------------------------------------------------------------------|---------------------------------------------------------------------------------------------------------|---------------------------------------------------------------------------------------------------------------------------------------------------------------|----------------------------------------------------------------------------------------------------------------------------------------------------------------------------------------------------------------------------------------------------------------------------------------------------------------------------------------------------------------------------------------------------------|
|   |                                                                | premotor cortex (PMd) based on multi-modal CBP combined with a detailed characterization                                    | (124 adults have DTI)                                                                                                   |                                                                        | clustering along with other connectivities                                                              |                                                                                                                                                               | performed and the reliability was validated with previous method and functional characterization<br>L: multimodality was obtained using three different datasets                                                                                                                                                                                                                                         |
| 4 | T. Fuchigami, Scientific Reports, 2018[4]                      | To use DTI-based registration for decoding of fMRI maps through zero-shot learning                                          | To classify the brain function from fMRI images (Total: 22) of a subject without having the subject's fMRI for training | The selective visual attention task assigned - left or right attention | To generate template DTI used in the perform registration of fMRIs as a primary step                    | SVM                                                                                                                                                           | A: The technique showed comparable accuracy with a decoder trained on single subject functional maps (5 subjects' DTI performed better than self-decoding)<br>L: small set, no external validation                                                                                                                                                                                                       |
| 5 | J. Kawahara, NeuroImage, 2017,[5]                              | To adapt of CNNs for edge-weighted networks and application of those to the human connectome.                               | Regress the menstrual age and neurodevelopmental outcome of pre-term infants (115 infants, 168 scans)                   | Preterm age and Bayley scales of infant and toddler development        | To compactly represent white-matter connectivity in terms of a graph                                    | ANN consisting of Novel edge-to-edge, edge-to-node and node-to-graph convolutional filters that leverage the topological locality of structural brain network | A: Proposed approach BrainNetCNN can predict an infant's postmenstrual age (Pearson's correlation:0.87) and outperforms existing ML approaches<br>L: prediction performance for neurodevelopmental outcome were relatively low, no external validation                                                                                                                                                   |
| 6 | L. Lin, Computer Methods and Programs in Biomedicine, 2016 [6] | Employment of DTI to explore the topological changes of whole-brain WM structural connectivity in the normal older subjects | Regress brain age of healthy older adults (112 scans)                                                                   | Age collected as part of the demographic information                   | To perform whole-brain tractography (needed for feature extraction) using the FA image derived from DTI | ANN with hybrid genetic algorithm (GA) and Levenberg-Marquardt (LM)                                                                                           | A: Quantification of the typical and atypical network organization of human brain and development of a biomarker for pre-symptomatic detection of future neurodegenerative diseases. Predicted brain age has a correlation of 0.8 with chronological age.<br>L: Slightly underestimation of brain age for subjects older than 70 years and a slightly overestimation of age for subjects younger than 55 |

|   |                                                      |                                                                                                                                                                                                   |                                                                                                                                                       |                                                                                                         |                                                 |                          |                                                                                                                                                                                                                                                                                                                           |
|---|------------------------------------------------------|---------------------------------------------------------------------------------------------------------------------------------------------------------------------------------------------------|-------------------------------------------------------------------------------------------------------------------------------------------------------|---------------------------------------------------------------------------------------------------------|-------------------------------------------------|--------------------------|---------------------------------------------------------------------------------------------------------------------------------------------------------------------------------------------------------------------------------------------------------------------------------------------------------------------------|
|   |                                                      |                                                                                                                                                                                                   |                                                                                                                                                       |                                                                                                         |                                                 |                          | years, lack of interpretability of ML, increased acquisition time of MRI, no external validation                                                                                                                                                                                                                          |
| 7 | D. Wang, Lecture Notes in Computer Science, 2014 [7] | To perform group connectivity of brain networks as previous researches focused in mean connectivity in patients                                                                                   | Novel brain connectivity network analysis method by was proposed to identify the consistent connectivity patterns from multiple subjects (50 healthy) | Two existing techniques used for comparison                                                             | To derive the brain network in terms of a graph | Multigraph Mix-Max Cut   | A: A novel brain connectivity network analysis method was proposed and that detected several important subnetwork modules, the performance in terms of weight (0.0983 vs 0.0911), fiber length (0.0592 vs 0.0551), and fiber number (0.0740 vs 0.0707) was better than mix-max cut.<br>L: No external validation          |
| 8 | H. Ullman, Journal of Neuroscience, 2014 [8]         | Use noisy multivariate data to investigate the potential for neuroimaging to predict future cognitive capacity performance on a visuospatial WM task in a longitudinal design                     | Regress future (2 years later) visuospatial working memory test scores in healthy individuals (323 subjects)                                          | VSWM scores collected from patients after two years of imaging data acquisition                         | To derive FA                                    | SVR + GLM                | A: Support in favor of unique role of neuroimaging was found and FA data of DTI was better (correlation 0.59) in predicting VSWM scores compared to blood oxygenation level- dependent data and gray matter volume data<br><br>L: No external validation, difficulties in excluding the confounding of non-linear effects |
| 9 | B. Mwangi, NeuroImage, 2013 [9]                      | Use whole-brain features to understand aging process, identify anatomical voxels (features) relevant in making accurate prediction and elucidate whether these maturation and ageing trajectories | Regress age of healthy human subjects (188 subjects)                                                                                                  | International Neuroimaging Data Sharing Initiative (INDI) online database provided age for the patients | To derive 4 parametric maps                     | Relevance Vector Machine | A: Age was predicted with low error. Pearson's correlation coefficient of 0.899 was obtained with RD<br>L: Cross-sectional design, no external validation                                                                                                                                                                 |

|    |                                               |                                                                                                                                                                           |                                                                                                           |                                          |                                                                         |                                                                                   |                                                                                                                                                                                                                                                                                                                                                                       |
|----|-----------------------------------------------|---------------------------------------------------------------------------------------------------------------------------------------------------------------------------|-----------------------------------------------------------------------------------------------------------|------------------------------------------|-------------------------------------------------------------------------|-----------------------------------------------------------------------------------|-----------------------------------------------------------------------------------------------------------------------------------------------------------------------------------------------------------------------------------------------------------------------------------------------------------------------------------------------------------------------|
|    |                                               | follow linear or non-linear paths.                                                                                                                                        |                                                                                                           |                                          |                                                                         |                                                                                   |                                                                                                                                                                                                                                                                                                                                                                       |
| 10 | R. Yun, IEEE EMBS, 2013 [10]                  | Use topological properties of brain networks and machine learning to predict scores                                                                                       | Regress cognitive performance scores of healthy aged individuals (96 subjects)                            | CASI Test scores                         | To derive the brain network in terms of graph                           | Linear regression, partial least square, Gaussian Process, Multi-layer perceptron | A: Cognitive performance score was predicted with low mean absolute error (5.8120 with linear regression, 6.25 with Gaussian process as top two performers in terms of the measure)<br>L: No external validation                                                                                                                                                      |
| 11 | Y. Wen, Magnetic Resonance Imaging, 2013 [11] | Use multi-channel fusion to improve tissue classification in DTI for robust performance against random noise and field inhomogeneity                                      | Segmentation of brain tissue in presence of random noise and magnetic field inhomogeneities (20 subjects) | Expert segmented ground truth            | To derive 14 parametric maps (including FA, MD, CL etc.)                | Fuzzy C-Means                                                                     | A: Proposed algorithm performed better segmentation than the existing ones with volume overlap over 84% for white matter, grey matter, and CSF.<br>L: Small dataset                                                                                                                                                                                                   |
| 12 | I. Maximov, Medical Image Analysis, 2012 [12] | Proposition of an advanced approach to remove noise by considering inhomogeneity of Rician noise distribution                                                             | Denoising of images having spatially varying Rician noise (one healthy)                                   | Established Noise Models                 | Serves as the input on which denoising is performed                     | Proposed technique BURST                                                          | A: Advanced approach for voxel-specific noise modeling was developed<br>L: Small set of real data                                                                                                                                                                                                                                                                     |
| 13 | Z. Hua, NeuroImage, 2012 [13]                 | Proposition of Bayesian local functional model (BFM) for analyzing different diffusion parameters of WM fiber bundles along with other covariates such as age and gender. | Clustering global anisotropy data of infants (128 healthy infants)                                        | Not Stated                               | To build DTI atlas, atlas fiber tractography and fiber parameterization | Proposed BFM                                                                      | A: The proposed model found complex heterogeneous spatio-temporal maturation patterns of WM fiber bundles. Data favored global clustering with an $\alpha = 5.34$<br>L: BFM cannot be used for DTI fiber correspondence across subjects, use of only b-spline bases. measurement error using Gaussian only, BFM is limited to diffusion properties along fiber bundle |
| 14 | A. Crippa, NeuroImage, 2011 [14]              | A technique to heuristically determine number of                                                                                                                          | Parcellation of supplementary motor area (SMA) and pre-SMA in                                             | MNI parcellation map and K-means results | To perform tractography used in the computation of                      | Force Directed Graph Layout                                                       | A: Proposed method provides insights about the connectivity                                                                                                                                                                                                                                                                                                           |

|    |                                       |                                                                                                                                                                                                                                                     |                                                                                                                                                      |                                                                                             |                                                            |                                                                                                                          |                                                                                                                                                                                                                                                                                                                                                                                                                 |
|----|---------------------------------------|-----------------------------------------------------------------------------------------------------------------------------------------------------------------------------------------------------------------------------------------------------|------------------------------------------------------------------------------------------------------------------------------------------------------|---------------------------------------------------------------------------------------------|------------------------------------------------------------|--------------------------------------------------------------------------------------------------------------------------|-----------------------------------------------------------------------------------------------------------------------------------------------------------------------------------------------------------------------------------------------------------------------------------------------------------------------------------------------------------------------------------------------------------------|
|    |                                       | intrinsically present clusters and investigate their organization in connectivity-based parcellation studies in brain and its application to applied our method to the parcellation of SMA (supplementary motor cortex) and pre-SMA, a brain region | healthy humans (13 healthy)                                                                                                                          |                                                                                             | cross-correlation matrix of the connectivity profiles      |                                                                                                                          | patterns of the premotor cortex. Overlap greater than 77% and 71% noted for the subjects for K=2 and K=3 clusters resp. L: Well defined clusters within SMA and pre-SMA across all subjects were not found.                                                                                                                                                                                                     |
| 15 | E. C. Robinson, NeuroImage, 2010 [15] | Identification of tracts in human brain that are related to aging                                                                                                                                                                                   | Classify healthy humans into two different age groups and identify tracts in humans that differ significantly across populations (96 healthy adults) | Age collected as part of demographic information provided in the publicly available dataset | To perform tractography and generate connectivity matrices | Maximum uncertainty linear discriminant analysis (MLDA) was applied on features projected on set of principal components | A: Proposed approach works in two cohorts with two types of age distribution and classification accuracy of 87.46% was obtained. L: more diffusion directions can be used, further experiments to assess the effect of gender on population, ROI from manually delineated atlases were used, errors during registration, segmentation, and tractography may generate false positive connections in tractography |

**sTable 2 Details of the studies that focused on mental health disorders cohorts**

| Serial Number | First Author, Publication Venue, Year, Reference | Unmet Need | ML Task Performed | Reference Standard for the Disease | Role of DTI | Machine Learning Model(s) Used | Accomplishments and Limitations (including what authors stated) |
|---------------|--------------------------------------------------|------------|-------------------|------------------------------------|-------------|--------------------------------|-----------------------------------------------------------------|
|---------------|--------------------------------------------------|------------|-------------------|------------------------------------|-------------|--------------------------------|-----------------------------------------------------------------|

|   |                                                                 |                                                                                                                                  |                                                                                                                                 |                                                                                       |                                         |                                            |                                                                                                                                                                                                                                                     |
|---|-----------------------------------------------------------------|----------------------------------------------------------------------------------------------------------------------------------|---------------------------------------------------------------------------------------------------------------------------------|---------------------------------------------------------------------------------------|-----------------------------------------|--------------------------------------------|-----------------------------------------------------------------------------------------------------------------------------------------------------------------------------------------------------------------------------------------------------|
| 1 | H. Zhuang, Neuroscience Letters, 2019 [16]                      | To explore the role of multimodal data for drug naive first-episode schizophrenia (FES)                                          | To classify FES and control (Total: 69, 40 drug-naive and 29 healthy)                                                           | Criteria using DSM-IV                                                                 | To extract DTI metrics                  | Sparse coding based feature selection, SVM | A: A multimodal classification method to discriminate FES from healthy controls was developed with accuracy of 84.29% and AUC of 81.64%<br>L: small set, imbalanced dataset                                                                         |
| 2 | X. Wang, European Psychiatry, 2019 [17]                         | To investigate the hierarchical structural connectomes' alterations of subnetworks in response to SSRI treatment in MDD patients | To classify pre-treatment, post-treatment MDD, and healthy controls (Total: 110 from 3 cohorts)                                 | DSM-IV and HAMD                                                                       | To extract DTI metrics                  | SVM                                        | A: A discriminative subnetwork was found for the classification with an accuracy of 86% for pre-treatment vs. healthy controls<br>L: small set, ML model not validated externally                                                                   |
| 3 | Y. Deng, Prog. Neuropsychopharmacol Biol. Psychiatry, 2019 [18] | To identify white-matter based biomarkers through machine learning for diagnosis of schizophrenia                                | Classify patients FES versus controls (Total 125: 65 FES, 60 controls)                                                          | DSM-IV criteria for schizophrenia and schizo-effective disorder, and confirmed by SCI | To derive DTI parameters from WM tracts | Random Forest                              | A: Validated in hold-out set with an accuracy 76% and discriminative inter-hemispheric and parieto-temporal connections were found<br><br>L: FES was medicated with psychotics, phenomena of cardiac gating was not considered in image acquisition |
| 4 | D. Alnæs, JAMA Psychiatry, 2018 [19]                            | To determine if structural connectivity in brain is a transdiagnostic phenotype for predicting                                   | To regress general psychopathology levels, age, and fluid intelligence using linked independent component analysis (Total: 729) | Age and data from behavioral phenotypes collected generated test battery              | To perform fiber tracking, TBSS         | Shrinkage linear regression                | A: Two major white matter tracts was found to be significantly related to cognitive and psychological factors. WM properties were associated with general                                                                                           |

|   |                                                               |                                                                                                                        |                                                                                                                                                                   |                                                                                                                                                                                |                                                         |                              |                                                                                                                                                                                                                                                                                                                                                                                   |
|---|---------------------------------------------------------------|------------------------------------------------------------------------------------------------------------------------|-------------------------------------------------------------------------------------------------------------------------------------------------------------------|--------------------------------------------------------------------------------------------------------------------------------------------------------------------------------|---------------------------------------------------------|------------------------------|-----------------------------------------------------------------------------------------------------------------------------------------------------------------------------------------------------------------------------------------------------------------------------------------------------------------------------------------------------------------------------------|
|   |                                                               | psychiatric symptoms                                                                                                   |                                                                                                                                                                   |                                                                                                                                                                                |                                                         |                              | psychopathology levels ( $r = 0.24$ ) and cognition ( $r = 0.39$ )<br>L: no external validation, follow-up assessment is needed for understanding the relevance of the results in long-term outcomes                                                                                                                                                                              |
| 5 | F. Deng, Prog Neuropsychopharmacol Biol Psychiatry. 2018 [20] | To combine neuroimaging methods with machine learning to obtain individual level predictions of BD and MDD             | Classify patients of BD, MDD, and controls (Total 112: 31 BD, 36 MDD, 45 healthy)                                                                                 | SCI for DSM-IV                                                                                                                                                                 | To derive DTI parameters used in representing WM tracts | SVM                          | A: Different abnormalities in specific segments of brain WM tracts may help in characterizing BD and the MDD. An accuracy of 68.33% was obtained using of FA tract profile of left anterior thalamic radiation<br><br>L: no external validation, used of deterministic tractography used, possibility of BD might have switched to MDD, controls not matched for age or education |
| 6 | P. Mikolas, BMC Psychiatry, 2018 [21]                         | To investigate whether machine learning applied to brain DTI data would differentiate between FES and Control patients | Classify FES patients from healthy controls<br><br>Regress chlorpromazine dose and symptom levels, from the multivariate patterns (Total 154: 77 FES, 77 healthy) | Patients with FES were recruited during their first psychiatric hospitalization, positive and Negative Syndrome Scale (PANSS) as a record of symptoms and chlorpromazine doses | To derive FA                                            | SVM, Kernel Ridge Regression | A: Provided a proof-of-concept using FA of WM early onset FES and HCs are separable with an accuracy of 62.34%<br><br>L: no external validation, presence of medicated patients                                                                                                                                                                                                   |
| 7 | S. H. Chu, IEEE EMBS, 2018 [22]                               | To discover changes connectivity and network                                                                           | Classify MDD patients from healthy controls (Total 79: 57 MDD, 27 healthy)                                                                                        | MDD diagnosis                                                                                                                                                                  | Anatomical connectivity and network measures            | SVM                          | A: Data-driven feature selection helped identifying neural correlates of MDD and                                                                                                                                                                                                                                                                                                  |

|   |                                 |                                                                                                                                                                                                                                                                                                     |                                                                                                                                                              |                                                                                                    |                                                                                                                         |                                |                                                                                                                                                                                                                                                                                                                                                                                 |
|---|---------------------------------|-----------------------------------------------------------------------------------------------------------------------------------------------------------------------------------------------------------------------------------------------------------------------------------------------------|--------------------------------------------------------------------------------------------------------------------------------------------------------------|----------------------------------------------------------------------------------------------------|-------------------------------------------------------------------------------------------------------------------------|--------------------------------|---------------------------------------------------------------------------------------------------------------------------------------------------------------------------------------------------------------------------------------------------------------------------------------------------------------------------------------------------------------------------------|
|   |                                 | topology from DTI measures using ML                                                                                                                                                                                                                                                                 |                                                                                                                                                              |                                                                                                    | from DTI metric (fiber count, AD, FA, MD, RD)                                                                           |                                | performed classification accuracy of 78%, sensitivity of 90.39%, and specificity of 79.66%<br><br>L: Small set, no external validation                                                                                                                                                                                                                                          |
| 8 | S. H. Chu, IEEE EMBS, 2018 [23] | To discover the effect of treatment in MDD with respect to connectivity and network topology from DTI measures using ML                                                                                                                                                                             | Classify treated versus untreated MDD (Total 52: 37 treated, 15 untreated)                                                                                   | MDD diagnosis followed by treatment history                                                        | Anatomical connectivity and network measures from DTI metric (fiber count, AD, FA, MD, RD) resulting in 138357 features | SVM                            | A: Data-driven feature selection helped identifying neural correlates of treated MDD and performed classification with 73% accuracy, 100% specificity, 100% precision.<br><br>L: Small set, no external validation                                                                                                                                                              |
| 9 | M.-J. Wu, NeuroImage, 2017 [24] | To circumvent the symptom-based categories specified DSM and identify distinct behavioral phenotypes using neurocognitive data and an unsupervised machine-learning technique. Second, using diffusion weighted neuroimaging scan data in a supervised manner to classify individuals into distinct | Cluster neurocognitive measurements to identify phenotypes and Classify cases to two types data-generated phenotypes BD and as HCs (Total 108: 70 BD, 38 HC) | Data-driven phenotypes generated from CANTAB for established bipolar disorder and healthy controls | To extract DTI parameters from TBSS skeleton                                                                            | K Means, LASSO and Elastic Net | A: Potential existence of two biologically distinct clinical phenotypes in BD compared to HC was found. FA and MD (TBSS-derived) predicted phenotype labels with 76% and 65% and phenotypes I and II were distinguished from HCs with 57% and 92% accuracy<br><br>L: no external validation for the classifier based on neuroimaging scans, binary classification was performed |

|    |                                                       |                                                                                                                                                                                                                                                                                 |                                                                                                          |                                                                                      |                                                                                   |              |                                                                                                                                                                                                                                                                                                                                                                                 |
|----|-------------------------------------------------------|---------------------------------------------------------------------------------------------------------------------------------------------------------------------------------------------------------------------------------------------------------------------------------|----------------------------------------------------------------------------------------------------------|--------------------------------------------------------------------------------------|-----------------------------------------------------------------------------------|--------------|---------------------------------------------------------------------------------------------------------------------------------------------------------------------------------------------------------------------------------------------------------------------------------------------------------------------------------------------------------------------------------|
|    |                                                       | phenotypes                                                                                                                                                                                                                                                                      |                                                                                                          |                                                                                      |                                                                                   |              |                                                                                                                                                                                                                                                                                                                                                                                 |
| 10 | T. M. Chaim-Avancini, Acta Psychiatr Scand. 2017 [25] | To apply large scale multimodal MRI in discriminating childhood-onset ADHD from controls                                                                                                                                                                                        | Classify childhood-onset ADHD versus HCs (Total 167: 67 ADHD, 66 HC)                                     | SCI for DSM-IV criteria in addition to ADHD related items for K-SADS-E               | To derive DTI parameters and extract ROIs based statistical and textures features | SVM          | A: Signature identified may have additional objective information and AUC of 71% was obtained for ADHD vs HC classification.<br><br>L: no external validation, 1.5 T MRI used                                                                                                                                                                                                   |
| 11 | G. Pfuhl, Hum Brain Mapp., 2016 [26]                  | To improve the understanding of WM microstructure in AN, the current study employed a global probabilistic tractography approach to analyze DTI data in a medication-free sample of both young acute (acAN) and recovered (recAN) female patients and pairwise age-matched HCs. | Cluster and classify HCs versus AN types (Total 129: 67 AN, 62 HC)                                       | acAN as per DSM-IV, recAN based on different clinical criteria,                      | To extract DTI parameters for WM based feature extraction                         | K-Means, SVM | A: Multivariate pattern classification showed potential to separate acAN from HC with an accuracy of 0.66<br><br>L: clustering was not successful, no external validation, current DTI techniques may miss subtle or more focal WM changes, varying duration of illness and recovery, bias in matching chronological age as delayed maturation of endocrine systems delay aging |
| 12 | K. Bi, Journal of Affective disorders, 2016 [27]      | To explore the relationship of functional connectivity (FC) based on MEG and                                                                                                                                                                                                    | To classify depression and control patients using FC-SC coupling (Total: 52, 26 depression, 26 controls) | SCI for DSM-IV, Hamilton Depression Rating scale, and Brief Psychiatric Rating Scale | To reconstruct fiber tracts                                                       | SVM          | A: Depression patients could be distinguished from controls for the entire time period of FC-SC coupling with best accuracy of 82.7% in the                                                                                                                                                                                                                                     |

|    |                                        |                                                                                                                                                                                     |                                                                                |                                                   |                                                                |                  |                                                                                                                                                                                                                               |
|----|----------------------------------------|-------------------------------------------------------------------------------------------------------------------------------------------------------------------------------------|--------------------------------------------------------------------------------|---------------------------------------------------|----------------------------------------------------------------|------------------|-------------------------------------------------------------------------------------------------------------------------------------------------------------------------------------------------------------------------------|
|    |                                        | structural connectivity (SC) from DTI for MDD patients                                                                                                                              |                                                                                |                                                   |                                                                |                  | acute rising phase of FC<br>L: small set, no external validation, more directions in DTI could have been considered                                                                                                           |
| 13 | S. Mas, PLoS One, 2016 [28]            | To integrate structural MRI, DTI, neuropsychological data, and genetic data to predict OCD early                                                                                    | To classify OCD and control patients (Total: 56, training set 38, test set 18) | DSM-IV diagnostic criteria for OCD                | To perform DTI metric extraction and VBM                       | SVM, Naive Bayes | A: Early onset OCD was predicted with accuracy of 65%, sensitivity 81%, specificity using multivariate tools in external validation set.<br>L: small set, OCD patients were medicated, single-center study                    |
| 14 | B. Mwangi, Psychiatry Res., 2015 [29]  | Primary objective of this study was to investigate the utility of DTI-derived measures (e.g. FA) in predicting individual PBD patients from healthy controls using a SVM algorithm. | Classify patients of PBD and HCs (Total 32: 16 PBD, 16 HC)                     | Diagnosis criteria for bipolar disorder by DSM-IV | To derive DTI parameters from WM tracts extracted using T1-MRI | SVM              | A: Potential ability of DW imaging measurements to distinguish PBD patients from HCs with accuracy of 78%<br><br>L: no external validation, small set, few patients were taking medications and had comorbidities present     |
| 15 | D. Peruzzo, J Neural Transm, 2015 [30] | Individual level prediction of FEP using multi-modal MRI                                                                                                                            | Classify FEP patients and HCs (Total 46: 23 FEP, 23 HC)                        | FEPs recruited from PICOS study                   | To extract 4 DTI parameters based on WM fiber bundle ROIs      | SVM, MKL         | A: Integration of multi-modal and multisource imaging data can classify FEP patients with high accuracy (90%) and right-hemisphere based prefronto-limbic network was found impaired in FEP.<br><br>L: small set, no external |

|    |                                                  |                                                                                                                                 |                                                                                                    |                                                                                                                                                                |                                                           |                 |                                                                                                                                                                                                                                                                                                                                                          |
|----|--------------------------------------------------|---------------------------------------------------------------------------------------------------------------------------------|----------------------------------------------------------------------------------------------------|----------------------------------------------------------------------------------------------------------------------------------------------------------------|-----------------------------------------------------------|-----------------|----------------------------------------------------------------------------------------------------------------------------------------------------------------------------------------------------------------------------------------------------------------------------------------------------------------------------------------------------------|
|    |                                                  |                                                                                                                                 |                                                                                                    |                                                                                                                                                                |                                                           |                 | validation, longitudinal approaches can potentially be used.                                                                                                                                                                                                                                                                                             |
| 16 | J. Arnedo, NeuroImage, 2015 [31]                 | Use generalized factorization method and non-negative matrix factorization to the FA-TBSS of schizophrenia and healthy patients | Clustering of SZ patients to identify heterogeneity of clinical behaviors (Total 83: 47 SZ, 36 HC) | DSM-IV criteria for schizophrenia, presence and severity of positive (psychotic) symptoms was assessed using the Scale for the Assessment of Positive Symptoms | To extract FA from TBSS skeleton                          | GFM-NMF         | <p>A: Reveals that SZ is a heterogeneous group of disorders which is established by different patterns of FA reductions associated with distinct clinical features, results were significant after Bonferroni correction in terms of t-test and f-test.</p> <p>L: small set, no external validation, phenotypic measurements can affect data quality</p> |
| 17 | J. Qin, Journal of Affective Disorders, 2015[32] | To study the topological properties of current major depressive disorder (cMDD), remitted MDD (rMDD), and HC                    | To classify cMDD, rMDD, and HC (Total: 73, 28 cMDD, 15 rMDD, 30 HC)                                | SCI for DSM-IV, Hamilton Depression Rating scale, and Brief Psychiatric Rating Scale                                                                           | To extract FA and MD                                      | SVM             | <p>A: Communication pathways were found to be associated with cMDD, rMDD and classification accuracy of 100% and 97.67% was obtained for cMDD and rMDD from HC and cMDD from rMDD</p> <p>L: small set, no external validation</p>                                                                                                                        |
| 18 | Y. Jin, Hum Brain Mapp. 2015 [33]                | Proposition of a novel multi-channel classification framework to identify infants at high-risk for ASD                          | Classify infants having high-risk versus low-risk of ASD (Total 80: 40 high-risk, 40 low-risk)     | Infants with older siblings having ASD and infants with no first-degree relative with ASD                                                                      | To derive WM connectivity networks for feature extraction | Multikernel SVM | <p>A: The proposed multiparameter multiscale performs better than single-scale network with an accuracy of 76% and AUC of 0.80</p> <p>L: small set, no external validation, acquisition</p>                                                                                                                                                              |

|    |                                           |                                                                                                                                                                       |                                                                            |                                                                                                                                   |                                                           |     |                                                                                                                                                                                                                                                                       |
|----|-------------------------------------------|-----------------------------------------------------------------------------------------------------------------------------------------------------------------------|----------------------------------------------------------------------------|-----------------------------------------------------------------------------------------------------------------------------------|-----------------------------------------------------------|-----|-----------------------------------------------------------------------------------------------------------------------------------------------------------------------------------------------------------------------------------------------------------------------|
|    |                                           |                                                                                                                                                                       |                                                                            |                                                                                                                                   |                                                           |     | parameters and reconstruction affect the features                                                                                                                                                                                                                     |
| 19 | F. Li, Hum Brain Mapp. 2014 [34]          | Use support vector machine to evaluate the white matter alterations in Obsessive Compulsive Disorder (OCD) patients                                                   | Classify OCD patients versus HCs (Total 56: 28 OCD, 28 HC)                 | SCI for DSM-IV                                                                                                                    | To derive WM guided FA values                             | SVM | <p>A: Showed spatially distributed discriminative WM abnormalities in individuals with OCD and OCD patients were identified with an accuracy of 84%</p> <p>L: Small set, no external validation, half of the patients had received medications</p>                    |
| 20 | J. Qin, Magn Reson Imaging, 2014 [35]     | To examine the potential value of diagnostic hubs in MDD patients and explore their pattern of disruption                                                             | Classify MDD patients versus HCs (Total 59: 29 MDD, 30 HC)                 | SCI for DSM-IV and the HDRS                                                                                                       | To derive connectivity matrix used for feature extraction | SVM | <p>A: Found evidence in the potential of hub as a valuable potential diagnostic measure for MDD and best accuracy obtained was 83.05%.</p> <p>L: small set, no external validation, use of deterministic tractography</p>                                             |
| 21 | W. Pettersson-Yeo, Psychol Med. 2013 [36] | Investigate the discriminative potential of genetic, sMRI, fMRI, DTI and/or cognitive data in the classification of FEP, ultra-high risk (UHR) and HC subjects at the | Classify UHR, FEP patients, and controls (Total 61: 19 FEP, 19 UHR, 23 HC) | DSM-IV criteria for FEP, UHC based on presence of psychotic symptoms (intermittent/attenuated) or having trait/state risk factors | To derive FA                                              | SVM | <p>A: Demonstrated ability of SVM and MRI to discriminate between different types of patients. Accuracy was greater than 65% with DTI for FEP vs HC and UHR vs HC</p> <p>L: FEP patients were medically and symptomatically stable at scanning, increased risk of</p> |

|    |                                                           |                                                                                                                                                                                                    |                                                                                                                          |                                                                                                                    |                                                            |                                                                                                                                              |                                                                                                                                                                                                                                                          |
|----|-----------------------------------------------------------|----------------------------------------------------------------------------------------------------------------------------------------------------------------------------------------------------|--------------------------------------------------------------------------------------------------------------------------|--------------------------------------------------------------------------------------------------------------------|------------------------------------------------------------|----------------------------------------------------------------------------------------------------------------------------------------------|----------------------------------------------------------------------------------------------------------------------------------------------------------------------------------------------------------------------------------------------------------|
|    |                                                           | individual level                                                                                                                                                                                   |                                                                                                                          |                                                                                                                    |                                                            |                                                                                                                                              | type 2 error, cross-section single center study, binary classification, no feature selection was employed                                                                                                                                                |
| 22 | M. Ingalhalikar, Lecture notes in Comp. Sc., 2012 [37]    | Understanding underlying data structure from DTI-extracted features and cognitive tests in an unsupervised manner for applications in autism spectrum disorder and schizophrenia                   | Clustering ASD and HCs (Total 46: 23 ASD, 23 HC)<br>Clustering SZ patients as separate cohorts (Total 54: 33 ASD, 21 HC) | Diagnosis                                                                                                          | To derive the connectivity matrix                          | Spectral clustering with similarity metric based variation of information from connectivity data and Euclidean distance for cognitive scores | A: Data clustering agreed with diagnostic labels in ASD (92% accuracy) and SZ datasets (78% accuracy).<br>L: small sets, no external validation                                                                                                          |
| 23 | P. Fang, PLoS One. 2012 [38]                              | Lack of clarity as to whether machine learning approaches will be able to extract whole-brain anatomical connectivity patterns to discriminate between depressed patients from controls accurately | Classify MDD patients and HCs (Total 49: 23 MDD, 26 HC)                                                                  | Unipolar recurrent MDD based on DSM-IV and evaluated by clinical psychologists for depression using SCI for DSM-IV | To perform tractography and derive the connectivity matrix | SVM                                                                                                                                          | A: Neurobiological diagnostic markers for MDD were found and abnormal cortical-limbic anatomical networks were found to be potentially responsible. Classification accuracy of 91.7% was obtained.<br>L: small sample size, low number of DTI directions |
| 24 | A. L. Fouque, Lecture notes in Comp. Sc Interv. 2011 [39] | Use of log-Euclidean metrics to incorporate the use of full tensor in the context of brain analysis                                                                                                | Regress Autism Diagnostic Interview-Revised scores for children and adolescents (30 patients)                            | Modified Autism Diagnostic Interview-Revised score                                                                 | To derive FA using log-Euclidean approach                  | Kernel Ridge Regression                                                                                                                      | A: Log-Euclidean framework improves over FA-analysis and brain-wide regression a cross-validated explained variance of 0.64                                                                                                                              |

|    |                                        |                                                                                                                     |                                                                                |               |                                              |     |                                                                                                                                                                                                                                                                            |
|----|----------------------------------------|---------------------------------------------------------------------------------------------------------------------|--------------------------------------------------------------------------------|---------------|----------------------------------------------|-----|----------------------------------------------------------------------------------------------------------------------------------------------------------------------------------------------------------------------------------------------------------------------------|
|    |                                        | through DTI                                                                                                         |                                                                                |               |                                              |     | L: Approach prone to over-fitting but seemed to recover with added deformation                                                                                                                                                                                             |
| 25 | M. Ingalhalikar, NeuroImage, 2011 [40] | Development of methodology for creating individual-level abnormality score based on region of interest from imaging | Classify ASD patients versus TD controls in children (Total 75: 45 ASD, 30 HC) | ASD Diagnosis | To derive 2 DTI parameters for specific ROIs | SVM | A: Distinction was made and FA and MD values of specific regions were found to be contributing to the abnormality score. 80% accuracy with 84% specificity and 74% sensitivity was obtained for the classification.<br>L: small set cannot capture entire disease spectrum |

**sTable 3 Details of the studies that focused on tumor-related studies**

| Serial Number | First Author, Publication Venue, Year, Reference | Unmet Need                                                                                                                                                   | Machine Learning Task Performed                                                  | Reference Standard for the Disease | Role of DTI            | Machine Learning Model(s) Used | Accomplishments and Limitations (including what authors stated)                                                                                                                                                                                                                |
|---------------|--------------------------------------------------|--------------------------------------------------------------------------------------------------------------------------------------------------------------|----------------------------------------------------------------------------------|------------------------------------|------------------------|--------------------------------|--------------------------------------------------------------------------------------------------------------------------------------------------------------------------------------------------------------------------------------------------------------------------------|
| 1             | A. Vamvakas, Physica Medica, 2019[41]            | To determine the importance multiparametric MR imaging based radiomic analysis and machine learning for understanding glioma heterogeneity in terms of grade | To classify glioma grades as high-grade or low-grade (Total: 40, 20 HGG, 20 LGG) | Diagnosis of HGG or LGG            | To extract DTI metrics | SVM                            | A: A comprehensive methodology for MRI-derived phenotype characterization of glioma grade was performed and linear SVM (using SMO implementation) with 95.5% accuracy, 95% sensitivity, 96% specificity<br>L: small sample size, no external validation, more imaging features |

|   |                                                         |                                                                                                                                      |                                                                                                                                                        |                                                                                                                                   |                                                                           |                                           |                                                                                                                                                                                                                                                                                                            |
|---|---------------------------------------------------------|--------------------------------------------------------------------------------------------------------------------------------------|--------------------------------------------------------------------------------------------------------------------------------------------------------|-----------------------------------------------------------------------------------------------------------------------------------|---------------------------------------------------------------------------|-------------------------------------------|------------------------------------------------------------------------------------------------------------------------------------------------------------------------------------------------------------------------------------------------------------------------------------------------------------|
|   |                                                         |                                                                                                                                      |                                                                                                                                                        |                                                                                                                                   |                                                                           |                                           | could be considered                                                                                                                                                                                                                                                                                        |
| 2 | L. S. Hu, American Journal of Neuroradiology, 2019 [42] | To use transfer-learning and MR imaging to quantify tumor cell density (TCD) in glioblastoma                                         | To regress tumor cell density using MR imaging (Total: 82 samples)                                                                                     | Histopathological analysis conducted by one neuropathologist                                                                      | To extract DTI metrics                                                    | Linear regression using transfer-learning | A: A collection of MR imaging features was found to predict TCD. Using multivariate modeling correlation of 0.88 was obtained<br>L: no external validation                                                                                                                                                 |
| 3 | S. Shrot, Neuroradiology, 2019[43]                      | To apply machine learning to distinguish among various types brain tumors using various MR sequences                                 | To classify among different types of brain tumor (Total: 141, 41 glioblastoma, 38 metastasis, 50 meningioma, 12 CNS)                                   | Pathological examination                                                                                                          | To extract DTI metrics                                                    | SVM                                       | A: High performance automatic tumor classification algorithm was developed. Classification accuracy for all binary classification > 90% , sensitivity > 81% (except CNS), specificity 91%<br><br>L: no external validation, ROI annotated manually, less samples CNS                                       |
| 4 | X. Leng, Cancer Imaging, 2019 [44]                      | To investigate if DTI data and machine learning can provide individual level predictions of NPC patients post-RT and normal controls | Classify different stages of post-therapy time elapse of nasopharyngeal carcinoma patients after radiotherapy and controls (Total: 147, 77 NPC, 67 HC) | Pathologically confirmed NPC underwent fractionated RT along and stages of post RT groups were formed according to the time lapse | To derive FA and extract automatic ROI-based features from WM connections | SVM                                       | A: WM regions and WM connection modes can be used as potential biomarkers for early diagnosis of RBI, classification accuracy as 82.5% of three post RT groups. FA based classification for was highest at 84.5% for post RT 0-6 months and controls<br>L: no external validation, NPC patients were given |

|   |                                                   |                                                                                                                                                        |                                                                                                |                                                  |                                                                                            |                                                                                                    |                                                                                                                                                                                                                                                                                    |
|---|---------------------------------------------------|--------------------------------------------------------------------------------------------------------------------------------------------------------|------------------------------------------------------------------------------------------------|--------------------------------------------------|--------------------------------------------------------------------------------------------|----------------------------------------------------------------------------------------------------|------------------------------------------------------------------------------------------------------------------------------------------------------------------------------------------------------------------------------------------------------------------------------------|
|   |                                                   |                                                                                                                                                        |                                                                                                |                                                  |                                                                                            |                                                                                                    | chemotherapy in different designs                                                                                                                                                                                                                                                  |
| 5 | F. Citak-Er, Computers in Bio. and Med, 2018 [45] | To evaluate the multi-parametric MRI extracted quantitative features for glioma grading                                                                | Classify low-grade and high-grade gliomas (Total 43: 15 low-grade, 28 high-grade)              | Histopathologic analysis                         | To derive 24 features including FA from the ROI                                            | SVM                                                                                                | A: ML based mutiparametric MRI features were able to predict tumor grade with classification accuracy of 93%, specificity 86.7% and sensitivity of 96.4%<br>L: Small set, proportion of low and high-grade patients differed, grouping grade-III and grade-IV in the same category |
| 6 | H. Akbari, Neuro-Oncology, 2018 [46]              | To determine EGFRvIII non-invariant non-invasively using diverse imaging features in GBM                                                               | To classify EGFRvIII status as positive or negative (Total: 129, discovery 75, replication 54) | Histopathological analysis                       | DTI metrics for microstructural feature extraction                                         | SVM                                                                                                | A: A specific radiomic signature of EGFRvIII identified which was verified in the replication cohort with an accuracy of 87% and AUC 0.86.<br>L: Single institutional data, EGFRvIII was evaluated as present versus absent                                                        |
| 7 | L. Chen, IEEE Trans. Med. Img., 2018 [47]         | Issues present data set associated with this study such as small sample size and complex, nonlinear (image) feature-to-(molecular) label relationship. | Classify both MGMT and IDH1 statuses in high-grade glioma patients (Total 47 subjects)         | Pathological (Biopsy-proven MGMT or IDH1 status) | To perform tractography and generate structural connectivity matrix for feature extraction | Proposed Multi-label Nonlinear Matrix Completion (MNMC) for jointly predicting MGMT and IDH status | A: Brain connectomics for HGG-prognosis can be used in a non-invasive manner. AUC of 0.787 for MGMT and 0.886 for IDH1 was obtained and compared better than existing techniques<br>L: absence of large patient populations with more heterogeneous data origins (for              |

|    |                                                                                |                                                                                                                                                                                                                                |                                                                                                   |                                   |                                                |                                                  |                                                                                                                                                                                                                                     |
|----|--------------------------------------------------------------------------------|--------------------------------------------------------------------------------------------------------------------------------------------------------------------------------------------------------------------------------|---------------------------------------------------------------------------------------------------|-----------------------------------|------------------------------------------------|--------------------------------------------------|-------------------------------------------------------------------------------------------------------------------------------------------------------------------------------------------------------------------------------------|
|    |                                                                                |                                                                                                                                                                                                                                |                                                                                                   |                                   |                                                |                                                  | generalization), limitation of the proposed ML method to work with missing feature values, limited set features used from rs-fmri, no external validation                                                                           |
| 8  | M. Soltaninejad, Computers in Bio. and Med., 2018 [48]                         | To segment brain tumour parts (core and oedema) using a novel multimodal MRI supervoxel based method                                                                                                                           | Automatic segmentation of brain tumor in images (11 patients had DTI in only one of the datasets) | Expert delineation of tumors      | To derive isotropic and anisotropic components | Random Forest                                    | A: A faster and reproducible method to segment brain tumor was developed with a detection sensitivity of 86%<br>L: small set, no external validation, limitation in segmenting small volume                                         |
| 9  | L. Chen, Medical Image Computing and Computer Assisted Intervention, 2017 [49] | As previous studies predicted either MGMT or IDH1 status alone by using a single-task machine learning technique, these studies combine potential relationship of these two molecular expressers to develop a prediction model | Classify MGMT and IDH1 status (two classes for each) in glioma patients (Total : 47)              | Biopsy-proven MGMT or IDH1 status | To extract DTI metrics, perform tractography   | Proposed Multi-label Inductive Matrix Completion | A: Pre-operative multimodal prediction of molecular biomarkers was shown to be feasible. AUC of 0.70 for MGMT and 0.885 for IDH1 was obtained and compared better than existing techniques<br>L: small set , no external validation |
| 10 | P. Eichinger, Scientific Reports, 2017[50]                                     | To integrate preoperative MRI using B0 and FA to identify IDH genotype in WHO grade II/III gliomas                                                                                                                             | To classify IDH genotype in gliomas (Total:79, training 59, testing 20)                           | Histopathological analysis        | To extract FA maps                             | ANN                                              | A: Classification accuracy and AUC in validation cohort was 92.1% and 0.91 resp.<br>L: small set, DTI with higher number of directions could be used, applied to WHO grade II/II gliomas                                            |

|    |                                               |                                                                                                                                                                                             |                                                                                                                                                                         |                                                                                                                                                                                                                       |                                                                                            |     |                                                                                                                                                                                                                                                                                 |
|----|-----------------------------------------------|---------------------------------------------------------------------------------------------------------------------------------------------------------------------------------------------|-------------------------------------------------------------------------------------------------------------------------------------------------------------------------|-----------------------------------------------------------------------------------------------------------------------------------------------------------------------------------------------------------------------|--------------------------------------------------------------------------------------------|-----|---------------------------------------------------------------------------------------------------------------------------------------------------------------------------------------------------------------------------------------------------------------------------------|
| 11 | L. Liu, Lecture notes in Comp. Sc., 2016 [51] | To utilize brain connectome to predict the treatment outcome for HGG patients                                                                                                               | Classify survival period as good versus bad in high-grade glioma patients (Total 68: 34 good, 24 bad)                                                                   | Patients who died within 650 days after surgery were labeled as “bad ” outcome group, and the remaining 34 patients who survived more than 650 days after the surgery were classified into the “good ” outcome group. | To perform tractography and generate structural connectivity matrix for feature extraction | SVM | A: Functional and structural networks provide complementary information and can improves the prediction accuracy to 75% compared to that if basic clinical information that provides 63.2%.<br>L: small set, more features can be provided to the model, no external validation |
| 12 | X. Qian, Medical Physics, 2016 [52]           | To develop an objective classification system for the classification of pseudo-progression (PsP) and true-progression (TTP) based on the longitudinal DTI and does not require segmentation | Classify PsP versus TTP of disease in glioblastoma multiform patients (Total: 35, 13 PsP, 22 TTP)                                                                       | The diagnosis of PsP and TTP was based on the follow-up imaging data and clinical experience of the physicians in charge.                                                                                             | To derive FA maps (longitudinal) used for 3D patch representation                          | SVM | A: analyzed longitudinal DTI without ROI segmentation to classify progression versus pseudo-progression with average accuracy and AUC of 86.7% and 92%<br>L: small set, no external validation                                                                                  |
| 13 | J. Zhang, Comp. in Bio and Med., 2016 [53]    | Extract volumetric information from DTI for GBM patients to identify pseudo-progression (PsP)                                                                                               | Classify PsP versus true-progression (TTP) of disease in glioblastoma multiforme patients (Two datasets<br>a. Total: 23, 9 PsP, 14 TTP<br>b. Total: 79, 23 PsP, 56 TTP) | PsP identification based on clinical and imaging data and the clinical experience of the physician                                                                                                                    | To derive FA maps used for extracting patches                                              | SVM | A: The method is not sensitive to tumor location and obtains good classification results (AUC: 0.87%) on tumor progression<br>L: small set, features from single DTI metric was used, no external validation                                                                    |
| 14 | H. Akbari, Neurosurgery, 2016 [54]            | To test the hypothesis that advanced pattern analysis and machine learning methods applied to multi-parametric MRI are able to                                                              | Classify edematous peritumoral tissue as recurring versus non-recurring in patients of WHO Grade                                                                        | Manually drawn ROI on pre-operative MRI to identify the region from which recurrence originated. Then edematous peritumoral regions                                                                                   | To extract features from 4 DTI parametric maps                                             | SVM | A: Visually imperceptible patterns from images helped in estimating the location of tumor recurrence with an AUC 0.84,                                                                                                                                                          |

|    |                                           |                                                                                                                                             |                                                                                                |                                                                                                                    |                                                                        |                                                             |                                                                                                                                                                                                                                                                   |
|----|-------------------------------------------|---------------------------------------------------------------------------------------------------------------------------------------------|------------------------------------------------------------------------------------------------|--------------------------------------------------------------------------------------------------------------------|------------------------------------------------------------------------|-------------------------------------------------------------|-------------------------------------------------------------------------------------------------------------------------------------------------------------------------------------------------------------------------------------------------------------------|
|    |                                           | quantitatively capture imaging variations and heterogeneity in edematous peritumoral tissue                                                 | IV glioblastoma who had future recurrence (two datasets a. 34 retrospective b. 34 prospective) | 5-20 mm were called non-recurring ROIs                                                                             |                                                                        |                                                             | sensitivity 91%, specificity 93%.<br>L: small set, no histopathologic ground truth from the infiltrated peritumoral areas.<br><br>Near and far peritumoral tissue are part of the algorithm and does not mean that distance is related to recurrence              |
| 15 | L. S. Hu, Plos One, 2015 [55]             | Integrating the diverse image-based phenotypes and rich textural data of multi-parametric MRI to quantify tumor content of biopsied samples | Classify biopsy samples of GBM patients as tumor-rich versus tumor-poor (82 biopsy samples)    | As per TCGA criteria for sample adequacy (the threshold of at least 80% tumor nuclei content to define tumor-rich) | To derive DTI parametric maps and isotropic and anisotropic components | LDA, DQDA, SVM                                              | A: model was validated and showed that multi-parametric MRI with an accuracy of 81.8% and texture analysis helped in the identification of tumor-rich biopsy targets<br>L: small set, other ML model will be required for a different threshold of nuclei content |
| 16 | R. Inano, NeuroImage: Clinical, 2014 [56] | To explore multiple DTI-based parameters for glioma grading                                                                                 | Classify high-grade versus low-grade in glioma patients (Total: 111, 36 LGG, 75 HGG)           | Histopathologically confirmed                                                                                      | To derive DTI parametric maps used for feature extraction              | SVM                                                         | A: Multiple DTI-based parameters from voxel-based DT-based clustered images can differentiate between HGG and LGGs with an AUC of 0.91<br>L: only DTI metrics were used, influence of distortions in voxel-based clustering, No external validation               |
| 17 | G. Yang, NMR in Biomedicine, 2014 [57]    | Parameters that describe tumour morphology and its irregularities can be adopted to differentiate                                           | Semi-automatically segment tumors and classify high-grade GBM                                  | Histopathological analysis                                                                                         | To derive isotropic and anisotropic components for performing semi-    | quadratic discriminant analysis (QDA), naïve Bayes (NB), k- | A: Morphological analysis-based ANN discriminated GBM and solitary metastasis with                                                                                                                                                                                |

|    |                                                  |                                                                                                                                                                                                                             |                                                                                         |                                         |                              |                                                                                                                    |                                                                                                                                                                                                                                                                                           |
|----|--------------------------------------------------|-----------------------------------------------------------------------------------------------------------------------------------------------------------------------------------------------------------------------------|-----------------------------------------------------------------------------------------|-----------------------------------------|------------------------------|--------------------------------------------------------------------------------------------------------------------|-------------------------------------------------------------------------------------------------------------------------------------------------------------------------------------------------------------------------------------------------------------------------------------------|
|    |                                                  | glioblastoma multiforme (GBM) from solitary metastasis (MET).                                                                                                                                                               | versus MET (Total 48: 30 GBM, 18 METs)                                                  |                                         | automatic tumor segmentation | nearest neighbour algorithm (k-NN), non-linear support vector machine (SVM), and artificial neural networks (ANN). | high cross-validation accuracy and AUC of 97.9% and 0.975 using ANN L: small set, semi-automatic, 3D features were not included                                                                                                                                                           |
| 18 | P. Svolos, Magnetic Resonance Imaging, 2013 [58] | Evaluate the potential of diffusion and perfusion MR to differentiate intracranial brain lesions such as high-grade glioma (HGG), low-grade glioma (LGG), atypical meningioma (aMNG), solitary metastases (MET)             | Classify intracranial brain lesions (Total 115, 20 LGG, 53 HGG, 24 aMNG, 18 MET)        | Histopathologically confirmed diagnosis | To derive FA                 | SVM                                                                                                                | A: Combination of diffusion and perfusion metrics helped in classification of intracranial brain lesions with an accuracy range 71%-95% L: No external validation                                                                                                                         |
| 19 | P. Svolos, Clinical Imaging, 2013 [59]           | Evaluate the joint potential of DWI, DTI, and DSI in identifying meningioma from other solitary metastases and determine the ability of diffusion and perfusion in the differential diagnosis of the aforementioned lesions | Classify atypical meningiomas and other brain tumors (Total 50: 8 aMNG, 15 GBM, 27 MET) | Histopathologically confirmed diagnosis | To derive FA                 | SVM, NB, K-NN                                                                                                      | A: diffusion metrics help to discriminate atypical meningiomas from glioblastoma and solitary metastasis. SVM present better classification ability with an accuracy of $0.90 \pm 0.04$ and F1-score 0.87 L: correction for contrast-agent extravasation not done, no external validation |

**sTable 4 Details of the studies that focused on trauma-related studies**

| Serial Number | First Author, Publication Venue, Year, Reference | Unmet Need                                                                                                                                                                               | Machine Learning Task Performed                                                                                                                                                                                                                        | Reference Standard for the Disease                                                                                                                                                          | Role of DTI                                                                                  | Machine Learning Model(s) Used                                         | Accomplishments and Limitations (including what authors stated)                                                                                                                                                                                                        |
|---------------|--------------------------------------------------|------------------------------------------------------------------------------------------------------------------------------------------------------------------------------------------|--------------------------------------------------------------------------------------------------------------------------------------------------------------------------------------------------------------------------------------------------------|---------------------------------------------------------------------------------------------------------------------------------------------------------------------------------------------|----------------------------------------------------------------------------------------------|------------------------------------------------------------------------|------------------------------------------------------------------------------------------------------------------------------------------------------------------------------------------------------------------------------------------------------------------------|
| 1             | V. M. Vergara, Journal of Neurotrauma, 2017 [60] | Compare resting state functional network connectivity and diffusion MRI for mTBI patients                                                                                                | Classify patients of mTBI versus healthy controls (Total 100: 50 mTBI, 50 control)                                                                                                                                                                     | Glasgow Coma Scale between 13 and 15 at first contact with medical staff, a maximum of 30 min loss of consciousness if present), and a maximum of 24 h post-traumatic amnesia (if present). | To extract FA values from white matter voxels                                                | SVM                                                                    | A: rsFNC was better than diffusion MRI in classifying mTBI in terms of accuracy (84.1% and 74.5%)<br>L: small set, no external validation, noise, high dimensionality, simple feature selection                                                                        |
| 2             | Z. S. Zheng, Human Brain Mapping, 2017 [61]      | To employ a multivariate approach to uncover which regions along the thalamic tracks are maximally informative in distinguishing among patient groups in traumatic brain injury patients | Classify among patients of mild Traumatic brain injury into two different levels of behavioral responses in minimally conscious states and Controls (Total 25: 10 vegetative state, 7 minimally conscious state minus, minimally conscious state plus) | Coma-recovery scale-revised                                                                                                                                                                 | To extract connectivity features values from 5-voxel sphere centered around each brain voxel | SVM                                                                    | A: DTI and machine learning have potential for diagnostic distinctions in DOC resulting from severe TBI with 100% accuracy using several thalamic tracts<br>L: small set, no external validation, and low number of diffusion directions                               |
| 3             | R. Goswami, Brain Struct Funct, 2016 [62]        | To use WM tract information from uncinate fasciculus to distinguish between concussed athletes from healthy                                                                              | Classify healthy controls and athletes with history of concussion using DTI extracted frontotemporal features (Total 36: 19 athletes, 17 controls)                                                                                                     | Neuropsychological assessment and neurological assessment                                                                                                                                   | To extract 4 DTI metrics in left and right hemisphere                                        | SVM, linear logistic net regression, sparse total variation classifier | A: Potential role of uncinate fasciculus (UF) in repeated concussion was revealed and UF mean and RD showed 79-84% sensitivity and specificity and 0.8 AUC<br>L: small set, no external validation, a cohort effect with possible self-selection to participate in the |

|   |                                               |                                                                                                                                                               |                                                                                                                                                                                                                                                                  |                                                                                                                                              |                                                                                |                  |                                                                                                                                                                                                                                                                                                                                                                                                               |
|---|-----------------------------------------------|---------------------------------------------------------------------------------------------------------------------------------------------------------------|------------------------------------------------------------------------------------------------------------------------------------------------------------------------------------------------------------------------------------------------------------------|----------------------------------------------------------------------------------------------------------------------------------------------|--------------------------------------------------------------------------------|------------------|---------------------------------------------------------------------------------------------------------------------------------------------------------------------------------------------------------------------------------------------------------------------------------------------------------------------------------------------------------------------------------------------------------------|
|   |                                               |                                                                                                                                                               |                                                                                                                                                                                                                                                                  |                                                                                                                                              |                                                                                |                  | study as well as restrictions on generalizability of the findings to others in this unique cohort of individuals with very high concussion and sub-concussion exposure, but not to people with a single or a few concussions.                                                                                                                                                                                 |
| 4 | E. D. Fagerholm, Brain, 2015 [63]             | Hypothesized that traumatic axonal injuries would most affect the structural connection hubs, defined in this study as nodes with high betweenness centrality | Classify patients with a previous history of TBI from healthy age-matched controls and regress the cognitive impairment commonly seen following TBI (Total 77: 52 TBI, 27 controls)                                                                              | Mayo Classification system based severe or moderate injury classification; radiologically confirmed microbleeds on a set of the TBI patients | To perform tractography and extract features from WM using connectivity matrix | SVM, Elastic Net | A: Combination of graph metrics were useful for explaining individual-level variability. Classification accuracy of 93.4% with cross-validation, correlation of 0.64 with information processing speed (with microbleeds). In replication cohort, highest correlation of 0.44 was found with information processing speed (controls and patients without microbleeds). L: Presence of partial volume effects, |
| 5 | P. J. Hellyer, Annals of Neurology, 2013 [64] | Application of machine learning to understand the traumatic axonal injury                                                                                     | Classify patients with traumatic axonal injury versus neurologically healthy controls and Regress neuropsychological outcome score for information processing speed, executive function, and associative memory in group of heterogeneous patients (70 patients) | Presence of microbleeds in imaging as determined by a neurologist in T2-MRI                                                                  | To extract 4 DTI parametric maps                                               | SVM, SVR,        | A: Classifiers showed high accuracy in discriminating patients with microbleeds from controls. Most accurate classifier using FA resulted in 94% accuracy. Correlation using FA and RD remained significant for information processing speed. L: Registration to be checked, patients have taking medications, FA                                                                                             |

|  |  |  |  |  |  |  |                                                                 |
|--|--|--|--|--|--|--|-----------------------------------------------------------------|
|  |  |  |  |  |  |  | and MO are dependent, cross-sectional analysis not longitudinal |
|--|--|--|--|--|--|--|-----------------------------------------------------------------|

**sTable 5 Details of the studies that focused on dementia-related studies**

| Serial Number | First Author, Publication Venue, Year, Reference               | Unmet Need                                                                                                                                             | Machine Learning Task Performed                                                                                                                                                                                                       | Reference Standard for the Disease                     | Role of DTI                                                 | Machine Learning Model(s) Used | Accomplishments and Limitations (including what authors stated)                                                                                                                                                                                                      |
|---------------|----------------------------------------------------------------|--------------------------------------------------------------------------------------------------------------------------------------------------------|---------------------------------------------------------------------------------------------------------------------------------------------------------------------------------------------------------------------------------------|--------------------------------------------------------|-------------------------------------------------------------|--------------------------------|----------------------------------------------------------------------------------------------------------------------------------------------------------------------------------------------------------------------------------------------------------------------|
| 1             | A. Wada, Magnetic Resonance in Medical Sciences, 2019 [65]     | To adapt machine learning to use structural connectome to discriminate Alzheimer's disease (AD), dementia with lewy bodies (DLB) from healthy patients | Classify patients of AD, DLB, and HCs (Total 48: 18 AD, 8 DLB and 22 HCs)                                                                                                                                                             | DSM-IV for AD and clinical diagnostic criteria for DLB | To generate the adjacency matrix of structural connectivity | CNN                            | A: MR connectome was able to identify dementia at an individual-level. Average precision and recall were 0.78 and 0.73 for AD, 0.94 and 0.65 in DLB, and 0.73 and 0.75 HCs<br>L: small number of subjects, use of deterministic tractography, no external validation |
| 2             | M. J. Knight, Journal of Magnetic Resonance Imaging, 2019 [66] | Using T2 relaxometry and DTI to explore the difference in states of certain brain structures in healthy controls, aMCI, and ADD                        | To classify aMCI, ADD, and HC (Total: 101, 25 aMCI, 14 ADD, and 62 HC)                                                                                                                                                                | Clinical criteria                                      | To extract DTI metrics (FA, MD, RD, AD)                     | SVM                            | A: More heterogeneous tissue states in aMCI and ADD was found using T2 relaxometry and DTI. Excellent sensitivity (79% and 94.5%) and specificity (85.6% and 86.1%) for aMCI and ADD<br>L: cohort imbalance, cross-sectional study, no external validation           |
| 3             | M.J.R.J. Bouts, Human Brain Mapping, 2019[67]                  | To determine the generalizability of MRI-based classification to detect MCI within a generalized population                                            | To perform the following (a) classify AD versus controls (b) mild AD and controls (c) moderate AD and controls (d) MCI and controls (e) models trained in (a), (b), (c) were tested in the cohort for (d) (Total:915, for a, b, c 250 | AD according to DSM-IV and NINCDS-ADRDA and MMSE score | To extract DTI metrics                                      | Elastic net regression         | A: Multiparametric MRI-based ML models in clinical cohort may translate to a general population cohort in a straight-forward manner for AD and mild-AD model with AUC of 0.60 and 0.57 resp.<br>L: only use of imaging in the                                        |

|   |                                            |                                                                                                                                               |                                                                                                    |                                                                                                                                             |                                                                                              |                                                     |                                                                                                                                                                                                                                                                                    |
|---|--------------------------------------------|-----------------------------------------------------------------------------------------------------------------------------------------------|----------------------------------------------------------------------------------------------------|---------------------------------------------------------------------------------------------------------------------------------------------|----------------------------------------------------------------------------------------------|-----------------------------------------------------|------------------------------------------------------------------------------------------------------------------------------------------------------------------------------------------------------------------------------------------------------------------------------------|
|   |                                            |                                                                                                                                               | samples and for d 665)                                                                             |                                                                                                                                             |                                                                                              |                                                     | models, only one type of classifier was tested                                                                                                                                                                                                                                     |
| 4 | G. W. Eldeeb, IEEE EMBS, 2018 [68]         | To derive and evaluate an Alzheimer's disease signature based on MD and FA                                                                    | To classify AD, EMCI, MCI, healthy controls (Total: 96, 35 AD, 6 EMCI, 25 LMCI, 31 HC)             | Tests employed in ADNI cohort                                                                                                               | FA and MD extraction                                                                         | SVM                                                 | A: SURF and SURF based features from DTI maps were able to perform multiclass classification (accuracy of 87% and 89% FA and MD) with improved performance compared to the state-of-the-art. L: small set, no external validation                                                  |
| 5 | R. A. Feis, NeuroImage Clinical, 2018 [69] | To combine machine learning with pre-symptomatic FTD mutation carriers to study individual classification of FTD-pathology at an early stage. | Classify pre-symptomatic frontotemporal dementia patients from controls (Total 103: 55 FTD, 48 HC) | Presence of three most common carriers                                                                                                      | To extract TBSS based features from DTI                                                      | LR                                                  | A: Separation of FTD mutation carriers can be from controls before symptom-onset and presence of FTD related pathological changes in WM. RD and WM density-based model achieved a classification AUC 0.68. L: small set, no external validation, sporadic bvFTD patients were used |
| 6 | E. E. Bron, Eur Radiology, 2017 [70]       | To investigate the added diagnostic value of ASL and DTI to structural MRI for classification of AD, FTD, and controls.                       | Classify patients of AD, FTD, and controls (Total 91: 24 AD, 33 FTD, 34 controls)                  | The reference standard was a diagnosis of AD or FTD established by consensus of a multidisciplinary team according to the clinical criteria | To extract VBM-Brain, CBF, and FA                                                            | SVM (binary and multi-class)                        | A: ASL and DTI augment structural MRI for multi-class classification AUC of 90% for. Binary AUCs were higher. L: small set, no external validation, diagnosis not based on histopathological data                                                                                  |
| 7 | T.M. Schouten, NeuroImage, 2017 [71]       | To assess the utility of machine learning in automated diagnosis of AD based on multimodal imaging                                            | Classify AD patients versus healthy controls (Total 250: 77 AD, 173 control)                       | Probable AD criteria for NINCDS-ADRDA and tested positive for CSF AD markers based on NIA-AA recommendations                                | To extract TBSS based features from DTI, independent component analysis (ICA) on DTI on TBSS | Logistic elastic net regression, Sparse Group LASSO | A: Evidence found to incorporate diffusion MR extracted features for AD classification. ICA-based FA features performed best with AUC of 0.92                                                                                                                                      |

|    |                                                                      |                                                                                                                                                                                                                     |                                                                                                                                                                                  |                                                                                                                                                                     |                                                             |               |                                                                                                                                                                                                                                                                                 |
|----|----------------------------------------------------------------------|---------------------------------------------------------------------------------------------------------------------------------------------------------------------------------------------------------------------|----------------------------------------------------------------------------------------------------------------------------------------------------------------------------------|---------------------------------------------------------------------------------------------------------------------------------------------------------------------|-------------------------------------------------------------|---------------|---------------------------------------------------------------------------------------------------------------------------------------------------------------------------------------------------------------------------------------------------------------------------------|
|    |                                                                      |                                                                                                                                                                                                                     |                                                                                                                                                                                  |                                                                                                                                                                     | based features, and graph measures from connectivity matrix |               | compared to 0.896 from Sparse Group LASSO. L: no external validation                                                                                                                                                                                                            |
| 8  | T. Maggipinto, Phys. in Med. And Bio., 2017 [72]                     | To perform a comparative study between nested and non-nested feature selection on the same data set.                                                                                                                | Classify patients of AD versus mild cognitive impairment (MCI) versus healthy control (HC) (Total 269: 150 training- 50 AD, 50 MCI and 50 HC, 119 testing- 39 AD, 40 MCI, 40 HC) | Probable AD criteria for NINCDS-ADRDA, MCI had memory concerns but no significant memory impairment                                                                 | To extract TBSS based WM features                           | Random Forest | A: Demonstrated the bias caused by non-nested feature selection and applied the selected features in another set. AUCs of 0.86 (HC vs AD) and 0.60 (HC vs MCI) was obtained with nested feature selection<br>L: Performance based on a single classifier was reported           |
| 9  | Y. Chen, Psych. Res.: NeuroImaging, 2017 [73]                        | To combine diffusivity and kurtosis by an ML-based approach in pathologic detection.                                                                                                                                | Classify AD versus HC (Total 56: 29 AD, 27 HC)                                                                                                                                   | NINCDS and Stroke-Alzheimer's Disease and Related Disorders Association criteria for AD + Cognitive scale assessment, normals have no condition for MCI or dementia | To extract features using DTI parameters from 23 ROIs       | SVM           | A: Enhanced understanding of DKI and the relationship between diffusivity and kurtosis in pathologic WM changes in Alzheimer's disease. Classification AUC with DKI was higher (99%) than that of DTI (95%)<br>L: Small set, no external validation, prodromal ADs not included |
| 10 | S. Ciulli, IEEE Journal of Biomed. And Health Informatics, 2016 [74] | To predict, on a single-patient basis, the impairment in executive functions (as measured by the TMT-B) in patients with MCI with small vessel disease (SVD) and investigate the brain substrate for these diseases | Classify normal and impaired cognitive performance in MCI with SVD (Total 40)                                                                                                    | TMT-B test scores scaled to ordinal values after age and education adjustment equivalent scores. These ES were subdivided into categories                           | To extract two DTI parameters from 50 ROIs                  | SVM           | A: Confirmed using feature ranking that MD in several WM regions are predictive of executive functions. MD features and SVM classified impaired performance with a sensitivity of (72.7% - 89.5%) and specificity (77.5%-80.0%)                                                 |

|    |                                              |                                                                                                                                                                                                                                                                                                                                         |                                                                                                                            |                                                                                                                                   |                                                                       |                         |                                                                                                                                                                                                                                                                                                              |
|----|----------------------------------------------|-----------------------------------------------------------------------------------------------------------------------------------------------------------------------------------------------------------------------------------------------------------------------------------------------------------------------------------------|----------------------------------------------------------------------------------------------------------------------------|-----------------------------------------------------------------------------------------------------------------------------------|-----------------------------------------------------------------------|-------------------------|--------------------------------------------------------------------------------------------------------------------------------------------------------------------------------------------------------------------------------------------------------------------------------------------------------------|
|    |                                              |                                                                                                                                                                                                                                                                                                                                         |                                                                                                                            |                                                                                                                                   |                                                                       |                         | L: small set, no external validation, feature selection not applied                                                                                                                                                                                                                                          |
| 11 | M. Dyrba, Human Brain Mapping, 2015 [75]     | To assess the utility of machine learning approaches for the automatic diagnosis of AD using various imaging modalities                                                                                                                                                                                                                 | Classify clinically probable AD versus HC (Total: 53, 28 AD, 25 HC)                                                        | Clinically probable AD according NINCDS-ADRCA + tested positive for CSF neurodegenerative markers based on NIA-AA recommendations | To extract mean gray matter tract intensity three DTI parametric maps | multiple kernel SVM     | A: Multimodal imaging data did not significantly improve classification accuracy compared mono-modal measures. Classification AUC 87% for DTI was obtained as a unimodal measure.<br>L: small set, no external validation, some atlas areas might be too large or too unspecific to detect group differences |
| 12 | M. Dyrba, Journal of Neuroimaging, 2015 [76] | To study DTI and SV, MK-SVM in assessing WM alterations of MCI subjects in a multicenter study                                                                                                                                                                                                                                          | To classify among two types of MCI and controls (Total: 95, CSF biomarker A-beta42+ 35, CSF biomarker A-beta42- 35, HC 25) | CSF biomarker amyloid-beta42                                                                                                      | To extract DTI metrics FA, MD, MO                                     | SVM                     | A. Accuracy rate of 77% was observed using MD parameter for MCI-Abeta42 subjects and controls,<br>L: Small set, no external validation                                                                                                                                                                       |
| 13 | S. Diciotti, IEEE EMBS, 2015 [77]            | The aim of this study was therefore the validation, comparison and implementation of machine learning techniques for multimodal classification between vascular mild cognitive impairment (VMCI) patients and healthy subjects and the discrimination, within the VMCI group, between patients with different cognitive performances as | Classify different levels of cognitive impairments in VMCI versus HC (Total: 87, 58 VMCI, 29 HC)                           | scores from MMSE exam and randomly chosen from an ongoing study on VMCI                                                           | To extract WM based feature vector                                    | SVM and Functional Tree | A: Improvement of multi-modality based ML compared to mono-modal ML. Highest AUC (93.1%) was obtained when WM DTI features were included for high-MMSE VMCI vs HC classification<br>L: small set, no external validation                                                                                     |

|    |                                                   |                                                                                                                                                                        |                                                                                                                       |                                                                                                                                                                                                           |                                                                                            |                         |                                                                                                                                                                                                                                                                                                                                                                           |
|----|---------------------------------------------------|------------------------------------------------------------------------------------------------------------------------------------------------------------------------|-----------------------------------------------------------------------------------------------------------------------|-----------------------------------------------------------------------------------------------------------------------------------------------------------------------------------------------------------|--------------------------------------------------------------------------------------------|-------------------------|---------------------------------------------------------------------------------------------------------------------------------------------------------------------------------------------------------------------------------------------------------------------------------------------------------------------------------------------------------------------------|
|    |                                                   | that that has not been done before.                                                                                                                                    |                                                                                                                       |                                                                                                                                                                                                           |                                                                                            |                         |                                                                                                                                                                                                                                                                                                                                                                           |
| 14 | Y. Xie, Journal of Alzheimer's Disease, 2015 [78] | Investigating the feasibility of integrating structural MRI and DTI to more accurately distinguish amnesic mild cognitive amnesia (aMCI) patients from controls.       | Classify Han Chinese aMCI with versus controls (Total 128: 64 aMCI, 64 HC)                                            | Consensus from two neurologists based on neuropsychological assessment evaluation, a battery of general neurological examinations, collateral and subject symptoms as well as functional capacity reports | To extract WM volume based features on DTI parametric maps                                 | SVM (classifier fusion) | A: Characterization of aMCI by a distributed pattern of GM and WM changes and classification AUC was 0.862<br>L: no external validation, more imaging modalities could be used, study based on cross-sectional datasets                                                                                                                                                   |
| 15 | D. Zhu, Human Brain Mapping, 2014 [79]            | Perform an assessment on MCI patients using structural and functional connectome                                                                                       | Classify patients with MCI versus controls (Dataset 1: 28 participants with 10 MCI patients and 18 healthy controls.) | NACC procedures and NINCDS-ADRDA diagnostic guidelines.                                                                                                                                                   | To extract Dense Individualized and Common Connectivity-based Cortical Landmarks (DICCCLs) | SVM                     | A: Functional connectome signatures formed using DTI-derived ROIs distinguished MCI from healthy aged controls with an accuracy of more than 95%.<br>L: No external validation, discarded DICCCLs which might be useful, dataset had more females than males.                                                                                                             |
| 16 | J. A. Pineda-Pardo, NeuroImage, 2014 [80]         | To accurately estimate functional connectivity thorough MEG between brain regions, and to quantify how much the structural connectivity contributes to the estimation. | Classify aMCI patients and healthy control (Total 81: 52 aMCI with 22 sdMCI and 30 mdMCI, 29 HC)                      | Neuropsychological battery of several tests                                                                                                                                                               | To extract connectivity matrix-based features                                              | KNN, LDA, SVM           | A: Using an anatomical prior improves the expressivity of the MEG-based model. LDA using structural connectivity-guided measures provide best accuracy of 86.27% for HC vs sdMCI classification<br>L: the MCI patients may convert to AD; restricted to alpha and beta bands of MEG; no universally agreed techniques on brain parcellation; quantification of structural |

|    |                                              |                                                                                                                                                                                                                                               |                                                                                                |                                                                      |                                                                  |                  |                                                                                                                                                                                                                                             |
|----|----------------------------------------------|-----------------------------------------------------------------------------------------------------------------------------------------------------------------------------------------------------------------------------------------------|------------------------------------------------------------------------------------------------|----------------------------------------------------------------------|------------------------------------------------------------------|------------------|---------------------------------------------------------------------------------------------------------------------------------------------------------------------------------------------------------------------------------------------|
|    |                                              |                                                                                                                                                                                                                                               |                                                                                                |                                                                      |                                                                  |                  | connectivity may contain errors; fiber crossing, bending or kissing are unresolved issues when using single DTI as a model of water diffusion; no leakage correction                                                                        |
| 17 | M. Li, Magnetic Resonance Imaging, 2014 [81] | Investigate tract-based feature extracted from DTI along with the volumetric features of gray matter for combination of ROI-based imaging markers from both atrophy pattern in gray matter and intensity based abnormalities in white matter. | Classify AD versus healthy people (Total: 36, 21 AD, 15 HC)                                    | probable AD diagnosis by NINCDS-ADRDA                                | To perform tractography and extract WM tract based features      | SVM              | A: Effectiveness of tract-based FA and the tract-based FA+ gray matter volumes-combined features were found with 94.3% accuracy, 95% sensitivity, 93.3% specificity<br>L: small set, no external validation                                 |
| 18 | M. Dyrba PLOS One, 2013 [82]                 | Evaluate the use of DTI as a biomarker in a multicenter setting accounting for effects of different MRI scanners                                                                                                                              | Classify AD patients versus HC in presence of scanner variability (Total: 280, 137 AD, 143 HC) | Clinically-probable AD according to NINDCS-ADRCA criteria            | To extract WM and GM based features from two DTI parametric maps | SVM, Naive Bayes | A: Machine learning allows scanner-independent classification of DTI datasets with pooled cross-validation accuracy of 80% with FA and 83% for MD<br>L: Patients in prodromal stages of AD were not considered in the dataset               |
| 19 | R. B. Patil, IEEE EMBS, 2013 [83]            | Investigate specific regions in white matter that are affected by AD                                                                                                                                                                          | Classify patients with AD disease versus controls (Total: 92, 34 AD, 58 HC)                    | MMSE scores along with other tests as mentioned in the ADNI protocol | To extract FA values for 50 ROIs                                 | AdaBoost         | A: Fornix of WM in brain was found to be affected by AD. Classification accuracy of 84.5% was obtained.<br>L: Better feature reduction techniques and better classifiers to improve the accuracy can be carried out, no external validation |
| 20 | S. Haller, American Journal of               | To apply DTI metrics to discriminate                                                                                                                                                                                                          | To classify various types of MCI (Total 66:                                                    | MMSE, Neuropsychological                                             | FA and TBSS                                                      | SVM              | A: Classification accuracy in each subgroup was                                                                                                                                                                                             |

|    |                                                      |                                                                                                                                                                                          |                                                                                                               |                                                                                                                                                          |                                                         |     |                                                                                                                                                                                                                                       |
|----|------------------------------------------------------|------------------------------------------------------------------------------------------------------------------------------------------------------------------------------------------|---------------------------------------------------------------------------------------------------------------|----------------------------------------------------------------------------------------------------------------------------------------------------------|---------------------------------------------------------|-----|---------------------------------------------------------------------------------------------------------------------------------------------------------------------------------------------------------------------------------------|
|    | Neuroradiology, 2013 [84]                            | among sd-aMCI, sd-fMCI, and md-aMCI                                                                                                                                                      | 18 sd-aMCI, 13 sd-fMRI, 35 md-aMCI)                                                                           | test battery determination                                                                                                                               |                                                         |     | more than 97%<br>L: small set, no external validation                                                                                                                                                                                 |
| 21 | W. Lee, Computers in Biology and Medicine, 2013 [85] | To perform early diagnosis of AD                                                                                                                                                         | To classify MCI and normal subjects (Total: 78, Discovery 40, Validation 38)                                  | Criteria for diagnosis in ADNI cohort                                                                                                                    | DTI metrics and perform TBSS                            | SVM | A: an accuracy of 100% was obtained on the independent test set<br>L: small set                                                                                                                                                       |
| 22 | C.-Y. Wee, NeuroImage, 2012 [86]                     | Combine DTI and rs-fmri at brain connectivity level for MCI diagnosis (not done at the time of writing the manuscript as per the authors)                                                | Classify mild cognitive impairment versus normal controls (Total: 27, 10 MCI, 17 Control)                     | a battery of general neuro-logical examination, neuropsychological assessment evaluation, collateral and subject symptom and functional capacity reports | To extract structural connectivity features             | SVM | A: Multimodal imaging provides improvement over single-modal imaging in identifying individuals with MCI with classification accuracy of 96.3% and AUC of 0.953<br>L: small-set, imbalanced data set, and lack of external validation |
| 23 | L. O'Dwyer, PLoS One, 2012 [87]                      | To apply DTI metrics to discriminate between healthy older subjects and MCI                                                                                                              | To classify healthy older adults and MCI (Total 73: 33 MCI, 40 Healthy older adults)                          | MMSE, Consortium to Establish a Registry for Alzheimer's Disease (CERAD) neuropsychological battery and not meeting specific criteria for dementia       | DTI parametric maps                                     | SVM | A: Using DTI and SVM, controls and MCI subjects were classified with high degree of (>90%) of sensitivity and specificity<br>L: small set, no external validation                                                                     |
| 24 | L. D'Dwyer, PLoS One, 2012 [88]                      | As ApoE4 is an established risk factor in Alzheimer's, identification of White matter tracts that can distinguish between carriers and non-carriers in young healthy adults is important | Classify ApoE4 carriers versus non-carriers in young healthy adults (Total: 44, 22 carriers, 22 non-carriers) | Genotype testing                                                                                                                                         | To extract TBSS based features from DTI parametric maps | SVM | A: Subtle WM differences are present in healthy young ApoE4 carriers and non-carriers and classification sensitivity and specificity are 90%<br>L: Limitations of tractography and lack of external validation                        |

**sTable 6 Details of the studies that focused on developmental disorders-related studies**

| Serial Number | First Author, Publication Venue, Year, Reference | Unmet Need | Machine Learning Task Performed | Reference Standard for the Disease | Role of DTI | Machine Learning Model(s) Used | Accomplishments and Limitations (including what authors stated) |
|---------------|--------------------------------------------------|------------|---------------------------------|------------------------------------|-------------|--------------------------------|-----------------------------------------------------------------|
|---------------|--------------------------------------------------|------------|---------------------------------|------------------------------------|-------------|--------------------------------|-----------------------------------------------------------------|

|   |                                              |                                                                                                                                                                                                                                         |                                                                                                                                        |                                                                                                                                |                                                                                      |                                |                                                                                                                                                                                                                                                                                                                              |
|---|----------------------------------------------|-----------------------------------------------------------------------------------------------------------------------------------------------------------------------------------------------------------------------------------------|----------------------------------------------------------------------------------------------------------------------------------------|--------------------------------------------------------------------------------------------------------------------------------|--------------------------------------------------------------------------------------|--------------------------------|------------------------------------------------------------------------------------------------------------------------------------------------------------------------------------------------------------------------------------------------------------------------------------------------------------------------------|
| 1 | C.-Y. Wee, Human Brain Mapping, 2017 [89]    | To investigate the heterogeneity of the neuroanatomical network among full-term neonates and to explore how neuroanatomical network can explain the variation of internalizing and externalizing behaviors in the first 4 years of life | Classify occurrence of internalizing and externalizing behavioral problems in neonates at 24 and 48 months of age (Total:120 neonates) | Child internalizing and externalizing behavior problems were assessed with maternal reports using the Child Behavior Checklist | To perform tractography and extract features from the anatomical connectivity matrix | SVM                            | A: Neural organization formed during fetal development could predict early childhood behavioral-emotional problems. Classification accuracy was 89.4%, specificity 0.765, and sensitivity 0.954<br>L: small set, white matter tract being unmyelinated in infants can cause low FA values and untimely termination of tracts |
| 2 | D. S. Tylee, NeuroImage: Clinical, 2017 [90] | To apply machine-learning methods in combination with diffusion imaging data to samples of individuals with 22q11.2DS.                                                                                                                  | Classify patients having 22q11.2 deletion syndrome versus controls (Total: 86, 56 22q11.2DS, 30 control)                               | Presence of the 22q11.2 deletion was confirmed with fluorescence in situ hybridization                                         | To perform tractography and extract WM tract features in terms of FA, AD, and RD     | SVM                            | A: WM-abnormalities in the middle and inferior longitudinal fasciculus (LF) were identified in patients. Average accuracy and AUC in repeated sub-sampled test sets were 0.85 and 0.89<br>L: small set, no independent validation, some tracts were excluded                                                                 |
| 3 | M. L. Krishnan, PNAS, 2017 [91]              | To investigate genetic influences on preterm brain development through linked diffusion MRI (d-MRI) and genomic data                                                                                                                    | Ranking of single-nucleotide polymorphism (SNPs) based genotypes in pre-term infants                                                   | Genomewide Genotyping                                                                                                          | To perform tractography and calculate weighted-connectivity matrix                   | Sparse Reduced Rank Regression | A: Previously unrecognized PPARG signaling has a role in cerebral development. SNPs in PPARG had a statistically                                                                                                                                                                                                             |

|   |                                                                 |                                                                                                                     |                                                                                                                          |                                                                           |                                                                                                     |                                       |                                                                                                                                                                                                                                         |
|---|-----------------------------------------------------------------|---------------------------------------------------------------------------------------------------------------------|--------------------------------------------------------------------------------------------------------------------------|---------------------------------------------------------------------------|-----------------------------------------------------------------------------------------------------|---------------------------------------|-----------------------------------------------------------------------------------------------------------------------------------------------------------------------------------------------------------------------------------------|
|   |                                                                 | and machine learning                                                                                                | (Total 272 infants)                                                                                                      |                                                                           |                                                                                                     |                                       | significant ( $p < 2.2 \times 10^{-7}$ ) high representation among top 100 SNPs<br>L: no external validation                                                                                                                            |
| 4 | Z. Cui, Human Brain Mapping, 2016, [92]                         | To investigate white matter anomalies in children using micro and macro-structural information and machine learning | Classify patients of developmental dyslexia versus controls in school-aged children (Total:61, 28 patients, 33 controls) | Standardized character recognition (CR) and word-list reading (WLR) tests | To perform tractography and extract five types of WM features based on volume and known DTI metrics | SVM, LR                               | A: Potential of neuroimaging features for identification of dyslexic patients were revealed. Classification accuracy of 83.61% was obtained by SVM.<br>L: small set, no external validation                                             |
| 5 | Y. G. Chimeno, Bio-Medical Materials and Engineering, 2014 [93] | Investigate fMRI, DTI extracted features with machine learning to classify dyslexic and monocular vision patients   | Classify children to control, dyslexic, monocular vision (MV) groups (Total 56)                                          | Vision tests, Neuropsychological tests                                    | To obtain FA values                                                                                 | SVM, ANN, KNN, K-means, LDA, AdaBoost | A: A new tool for the classification of subjects with dyslexia and monocular vision was found with ANN performing at an accuracy of 94.87% for distinguishing between MV and dyslexia<br>L: small set, cohort and ML was not elaborated |

**sTable 7 Details of the studies that focused on movement disorders-related studies**

| Serial Number | First Author, Publication Venue, Year, Reference | Unmet Need | Machine Learning Task Performed | Reference Standard for the Disease | Role of DTI | Machine Learning Model(s) Used | Accomplishments and Limitations (including what authors stated) |
|---------------|--------------------------------------------------|------------|---------------------------------|------------------------------------|-------------|--------------------------------|-----------------------------------------------------------------|
|---------------|--------------------------------------------------|------------|---------------------------------|------------------------------------|-------------|--------------------------------|-----------------------------------------------------------------|

|   |                                                                 |                                                                                                                                                                               |                                                                                                                           |                                                                                                                              |                                                                            |             |                                                                                                                                                                                                                                                                                                                   |
|---|-----------------------------------------------------------------|-------------------------------------------------------------------------------------------------------------------------------------------------------------------------------|---------------------------------------------------------------------------------------------------------------------------|------------------------------------------------------------------------------------------------------------------------------|----------------------------------------------------------------------------|-------------|-------------------------------------------------------------------------------------------------------------------------------------------------------------------------------------------------------------------------------------------------------------------------------------------------------------------|
| 1 | H. Lei, IEEE Journal of Biomed. and IEEE Informatics, 2019 [94] | To design a unified multi-task feature selection model to explore various relations among features, samples, and response variables of PD, SWEDD, and normal controls (NC)    | Classify PD and controls and regression for clinical score prediction of four tests (Total: 238, 142 PD, 34 SWEDD, 62 NC) | Recruited from PPMI cohort, and test scores for depression (GDS), sleep (ESS), olfaction (UPSIT), and cognition tests (MoCA) | Extract of 116 features from MD                                            | SVM and SVR | A: A joint multi-task feature selection was developed for classification (AUC: 96.37% for NC vs. SWEDD, 95.39 for PD vs. SWEDD) and regression (RMSE: 0.583 for MoCA in NC vs. PD).<br>L: only MR was used, only SVM was used, usage of handcrafted features                                                      |
| 2 | L. Jin, Behavioural brain Research, 2019 [95]                   | To discover imaging features of Parkinson's diseases (PD) and scans without dopaminergic (SWEDD)                                                                              | Classify PD versus SWEDD (Total: 54, 26 PD, 28 SWEDD)                                                                     | Recruited from PPMI cohort                                                                                                   | To extract connectivity between regions and calculate voxel-based features | SVM         | A: SVM was used on DTI to successfully classify between PD and SWEDD with the highest accuracy of 81.25%<br><br>L: small set, no external validation, no healthy control group,                                                                                                                                   |
| 3 | R. Morisi, Parkinsonism and Related Disorders, 2018 [96]        | Improve automatic diagnostic classification of degenerative parkinsonism (a definite diagnosis can be achieved only post mortem) at an individual level using imaging markers | Classify patients with different forms of Parkinsonism (Total: 85)                                                        | Clinical (clinical diagnosis performed by neurologists according to pre-defined criteria)                                    | To extract DTI metrics from brain regions                                  | SVM         | A: Multimodal imaging (highest accuracy 98%, sensitivity 91%, specificity 100% for PSP vs. all) and graph-based features-based (highest accuracy 98%, sensitivity 91%, specificity 100%) for PSP vs. all SVM was useful in determining PD<br>L: Limited size of the sample, lack of postmortem definite diagnosis |

|   |                                                      |                                                                                                                                                    |                                                                                                                                                                                                                                            |                                                                                                                                                                                                                                                                                                                                                |                                                                 |                                      |                                                                                                                                                                                                                                                                                               |
|---|------------------------------------------------------|----------------------------------------------------------------------------------------------------------------------------------------------------|--------------------------------------------------------------------------------------------------------------------------------------------------------------------------------------------------------------------------------------------|------------------------------------------------------------------------------------------------------------------------------------------------------------------------------------------------------------------------------------------------------------------------------------------------------------------------------------------------|-----------------------------------------------------------------|--------------------------------------|-----------------------------------------------------------------------------------------------------------------------------------------------------------------------------------------------------------------------------------------------------------------------------------------------|
| 4 | G. Du, American Journal of Neuroradiology, 2017 [97] | Comparing the pattern of DTI and R2* changes among the different parkinsonian diseases and a control group in multiple ROIs using machine learning | Classify patients of Parkinson's disease, multiple system atrophy, progressive supranuclear palsy, and healthy controls (Total: 106, 35 Parkinson disease, 16 multiple system atrophy, and 19 progressive supranuclear palsy, 36 controls) | Patient diagnoses were initially established according to published criteria by a movement disorder specialist and updated (August 2016) before the analysis of the current data according to the most recent clinical assessment and postmortem pathology if available (5 PD and 3 PSP cases were confirmed by postmortem pathology results). | To extract FA and MD metrics from selected regions of the brain | LR (6 scenarios to test)             | A: Combination of DTI and transverse relaxation rate for PD vs. PsP provided best AUC of 0.99<br>L: no external validation, patients were under medication, only 8 had postmortem confirmed diagnosis, case-control study, data was collected on patients under anti-parkinsonian medications |
| 5 | Y. Liu, Statistics in Medicine, 2017 [98]            | To develop a data-driven machine learning method to assist personalized recommendation for screening and diagnostic practices                      | Classify Parkinson disease patients versus controls (Total: 50 with DTI)                                                                                                                                                                   | United Kingdom Brain Bank criteria                                                                                                                                                                                                                                                                                                             | To extract FA values from WM and parietal lobe                  | Weighted SVM                         | A: Superior performance of individualized rules with an AUC of 93.7%<br>L: Small set, no external validation                                                                                                                                                                                  |
| 6 | H. Liu, Journal of Neuroscience Methods, 2016 [99]   | To propose the employment of the FCP to the biomarker identification problem in PD for the first time.                                             | Feature selection for identification of biomarker of Parkinson's disease (Total: 65,                                                                                                                                                       | PD diagnosis was confirmed by a movement disorder specialist according to                                                                                                                                                                                                                                                                      | To extract FA and MD values from brain regions                  | Folded concave penalized (FCP) model | A: Clinically relevant MRI markers UPSIT were identified by the approach and FCP on clinical and MRI features achieved an AUC of 0.99                                                                                                                                                         |

|   |                                                           |                                                                                                                                                                                                |                                                                                                                                   |                                                                                                                                                                            |                                                         |     |                                                                                                                                                                                                                                               |
|---|-----------------------------------------------------------|------------------------------------------------------------------------------------------------------------------------------------------------------------------------------------------------|-----------------------------------------------------------------------------------------------------------------------------------|----------------------------------------------------------------------------------------------------------------------------------------------------------------------------|---------------------------------------------------------|-----|-----------------------------------------------------------------------------------------------------------------------------------------------------------------------------------------------------------------------------------------------|
|   |                                                           |                                                                                                                                                                                                | 34 PD, 31 HC)                                                                                                                     | the UK brain bank clinical diagnosis criteria                                                                                                                              |                                                         |     | L: small set, no external validation, minimal convex penalty method used is affected by collinearity                                                                                                                                          |
| 7 | A. Cherubini, Movement Disorders, 2014 [100]              | To distinguish patients of PD and progressive nuclear palsy (PSP) using DTI                                                                                                                    | To classify PSP and PD patients (Total: 78, 21 PSP, 57 PD)                                                                        | Neurological examinations and clinical assessments using the Unified Parkinson Disease Rating Scale-Motor Examination (UPDRS-ME) and the Hoehn and Yahr (H&Y) rating scale | To extract DTI metrics                                  | SVM | A: Computer-based SVM analysis on VBM-based GM atrophy and diffusion measures can help in distinguish PD from PSP patients with 90% sensitivity and 96% specificity<br>L: small set, no external validation, clinical criteria for PD and PSP |
| 8 | A. Cherubini, Movement Disorders, 2014 [101]              | To distinguish patients with tremor-dominant Parkinson's disease (tPD) from patients with essential tremor with rest tremor (rET)                                                              | To classify tPD and rET patients (Total: 30. 15 rET, 15 tPD)                                                                      | Clinical criteria for tPD                                                                                                                                                  | To extract DTI metrics                                  | SVM | A: A combination of VBM and DTI analyses showed 100% accuracy for the differentiation of patients with rET from those with tPD<br>L: small set, no external validation                                                                        |
| 9 | S. Haller, American Journal of Neuroradiology, 2012 [102] | Detection of idiopathic PD versus other atypical forms of Parkinsonism including multisystem atrophy and progressive supranuclear palsy is challenging as visually detectable brain MR imaging | Classify PD patients versus healthy patients in a cohort of consecutive suspected PD patients (Total: 40, 17 PD, 23 suspected PD) | PD group, a diagnosis of PD was made in the presence of typical, asymmetric, and levodopa-responsive Parkinsonism meeting the UK Parkinson's Disease Society Brain Bank    | To extract TBSS based features from DTI parametric maps | SVM | A: SVM based DTI provides improved detection of PD with an accuracy of up to 97%<br>L: retrospective, small set and lack of external validation set                                                                                           |

|  |  |                                |  |                                                                                                      |  |  |  |
|--|--|--------------------------------|--|------------------------------------------------------------------------------------------------------|--|--|--|
|  |  | differences may not be present |  | criteria, including at least 2 supportive criteria such as slow progression or peak-dose dyskinesia. |  |  |  |
|--|--|--------------------------------|--|------------------------------------------------------------------------------------------------------|--|--|--|

**sTable 8 Details of the studies that focused on other neurological disorders-related studies**

| Serial Number | First Author, Publication Venue, Year, Reference      | Unmet Need                                                                                                                                | Machine Learning Task Performed                                                                                                           | Reference Standard for the Disease                                                                                | Role of DTI                                     | Machine Learning Model(s) Used                                | Accomplishments and Limitations (including what authors stated)                                                                                                                                                                                                                                                                                        |
|---------------|-------------------------------------------------------|-------------------------------------------------------------------------------------------------------------------------------------------|-------------------------------------------------------------------------------------------------------------------------------------------|-------------------------------------------------------------------------------------------------------------------|-------------------------------------------------|---------------------------------------------------------------|--------------------------------------------------------------------------------------------------------------------------------------------------------------------------------------------------------------------------------------------------------------------------------------------------------------------------------------------------------|
| 1             | B. C. Munsell, Brain and Language, Review, 2019 [103] | To find the neuronal network associated with the naming performance in patients with medical refractory TLE and left hemisphere dominance | To select features from connectome that related to language scores and regress the language performance score of the patients (Total: 24) | Boston Diagnostic Aphasia Examination (BDAE)                                                                      | To perform tractography and generate connectome | Sparse Learning (feature selection), SVR (for regression)     | A: Naming impairments were associated with structural preservation of sub-network of gray matter regions located primarily in the temporal and frontal areas. Low errors (MSE<0.05) were obtained in predicting the scores of all six tests and results were interpreted clinically.<br>L: small set, no external validation, lack of a control group. |
| 2             | C.-H. Park, Neuroscience Letters, 2019 [104]          | Address conflicting findings on the relationship between seizure frequency                                                                | Classify in temporal lobe epilepsy patients having high versus low frequency of seizures and                                              | Clinical (criteria of the International League Against Epilepsy) for epilepsy detection, Engel classification for | To extract FA of WM tracts                      | Random Forest (binary classification), Model-based clustering | A: TLE subdivision achieved inferior classification (accuracy: 69%-71%) compared to                                                                                                                                                                                                                                                                    |

|   |                                              |                                                                                                                                                                          |                                                                                                                                                                                   |                                                                                               |                                                                             |     |                                                                                                                                                                                                                                                                                          |
|---|----------------------------------------------|--------------------------------------------------------------------------------------------------------------------------------------------------------------------------|-----------------------------------------------------------------------------------------------------------------------------------------------------------------------------------|-----------------------------------------------------------------------------------------------|-----------------------------------------------------------------------------|-----|------------------------------------------------------------------------------------------------------------------------------------------------------------------------------------------------------------------------------------------------------------------------------------------|
|   |                                              | and neuroanatomical damage                                                                                                                                               | Classify TLE patients and controls (Total: 87, 42 TLE, 45 HC)                                                                                                                     | seizure frequency according to seizure diaries six months before acquisition of MRIs          |                                                                             |     | TLE detection (accuracy: 75%-80%)<br>L: small sample size, no external validation                                                                                                                                                                                                        |
| 3 | E. Moulton, NeuroImage: Clinical, 2019 [105] | To explore DTI-derived parameter maps, lesion segmentations, and machine learning for function outcome post-stroke                                                       | To classify 3-month post-stroke outcome into good and bad categories using imaging at 24h post-stroke and baseline clinical variables (Total 87: 61 good outcome, 26 bad outcome) | Clinical assessment using mRS at 3 months post-stroke                                         | DTI metrics extraction                                                      | SVM | A: Study was the first to use whole brain DTI data in a multivariate framework for classifying functional outcome with an accuracy of 82.8%<br>L: Small set, no external validation, all lesions were located in the same hemisphere, analysis restrained to white matter                |
| 4 | K. Mithani, Annals of Neurology, 2019 [106]  | To predict the response of vagus nerve stimulation (VNS) response using diffusion tensor imaging and MMEG recording to inform patient selection for epilepsy in children | To classify VNS treatment outcome response (Total: 56, discovery = 38, validation = 18)                                                                                           | Post-therapy seizure reduction by more than 50% treated as responders, rest as non-responders | To extract DTI metrics, perform TBSS inform atlas-guided beamforming in MEG | SVM | A: The classification was validated in using independent test set from three institutions with an accuracy of 83.3%, sensitivity of 85.7%, specificity of 75%<br>L : small set, dichotomous response classification, more proportion of responders in the discovery and validation sets, |

|   |                                               |                                                                                                                                                                             |                                                                                                                                           |                                                           |                                                               |                           |                                                                                                                                                                                                                                                                                                                                                                    |
|---|-----------------------------------------------|-----------------------------------------------------------------------------------------------------------------------------------------------------------------------------|-------------------------------------------------------------------------------------------------------------------------------------------|-----------------------------------------------------------|---------------------------------------------------------------|---------------------------|--------------------------------------------------------------------------------------------------------------------------------------------------------------------------------------------------------------------------------------------------------------------------------------------------------------------------------------------------------------------|
|   |                                               |                                                                                                                                                                             |                                                                                                                                           |                                                           |                                                               |                           | retrospective analysis                                                                                                                                                                                                                                                                                                                                             |
| 5 | S. Payabvash, NeuroImage Clinical, 2019 [107] | To use DTI metrics and machine learning in sensory processing disorder (SPD)                                                                                                | To classify SPD versus typically developing controls (TDC) (Total: 85, 44 SPD, 41 TDC)                                                    | Parent reported Sensory Profile                           | DTI metrics and tractography                                  | Naive Bayes, RF, SVM, ANN | <p>A: First in literature to first in the literature to machine learning algorithms on DTI microstructural and connectivity information for classification of children with SPD. Highest classification accuracy of 77.5% (73.8 sensitivity, 81.6% specificity) was provided by RF.</p> <p>L: small set, heterogeneity in SPD patients, no external validation</p> |
| 6 | E. Gleichgerricht, Epilepsia, 2018 [108]      | To evaluate if deep learning could identify sets of connectome features and their combinations, associated with surgical outcomes from mesial temporal lobe epilepsy (mTLE) | Classify post-surgical outcomes of disabling seizures versus being seizure-free in mTLE patients (Total: 50, 14 seizure, 36 seizure-free) | Surgical outcome assessed by Engel Surgical Outcome Scale | To perform tractography and calculate the connectivity matrix | ANN                       | <p>A: Deep learning was powerful to approach to provide individual-level identification of seizure outcomes after surgery with a PPV of <math>88\pm 7\%</math> and NPV of <math>79\pm 8\%</math></p> <p>L: small set, retrospective, one type of several parcellations used, no external validation</p>                                                            |

|   |                                                |                                                                                                                                          |                                                                                                                                                                                                                           |                                                                                                                          |                                                                   |                                                      |                                                                                                                                                                                                                                                                                                                 |
|---|------------------------------------------------|------------------------------------------------------------------------------------------------------------------------------------------|---------------------------------------------------------------------------------------------------------------------------------------------------------------------------------------------------------------------------|--------------------------------------------------------------------------------------------------------------------------|-------------------------------------------------------------------|------------------------------------------------------|-----------------------------------------------------------------------------------------------------------------------------------------------------------------------------------------------------------------------------------------------------------------------------------------------------------------|
| 7 | M. Zurita, NeuroImage: Clinical, 2018 [109]    | To develop classifiers based on DTI and fMRI data that can identify areas of the brain that may help to better characterize the disease. | Classify patients of relapsing-remitting multiple sclerosis versus healthy controls<br>Classify patients of relapsing-remitting multiple sclerosis with different degree of disability (Total 157: 107 RRMS, 50 controls) | MS diagnosis according to McDonald's criteria and further separation of MR using EDSS (expanded disability status scale) | To extract FA and perform tractography                            | SVM                                                  | A: Classifiers developed were able to discriminate between healthy and diseased patients with an accuracy level of $89\% \pm 2\%$ .<br>Classification accuracy for disease levels was $63\% \pm 5\%$<br>L: combined classifier did not use FA, cohort included levels of low disability, no external validation |
| 8 | P. N. Taylor, NeuroImage: Clinical, 2018 [110] | To investigate change in connectivity metric in context of epilepsy surgery                                                              | Classify outcomes (seizure free versus not seizure free) in patients who underwent temporal lobe surgical resection (Total:53, 36 seizure free, 17 with seizure)                                                          | Postsurgical outcome assessed as per ILAE classification of surgical outcomes at 12 months after surgery                 | To perform tractography and generate connectivity matrix          | SVM                                                  | A: Brain network changes using between pre-operative and post-operative MRI predict seizure outcome with 79% accuracy and 65% specificity.<br>L: small set, no external validation, flipped connectivity matrices, two raters drew the resection masks                                                          |
| 9 | Y. Wang, Epilepsy and Behavior, 2018 [111]     | Existing FCD segmentation techniques are affected by class imbalance problem, so Gaussian processes for ML classifier was used           | Detection of gray and white matter abnormalities of focal cortical dysplasia in extratemporal lobe epilepsy (Total: 12)                                                                                                   | Radiological (a neuroradiologist manually drew lesions)                                                                  | To extract DTI metrics from cortical gray matter and white matter | Gaussian process for Machine Learning (GPML) and SVM | A: Multimodal-MRI based GPML achieved promising performance towards the detection of FCD with mean AUC of 0.76<br>L: Wide-age distribution of                                                                                                                                                                   |

|    |                                            |                                                                                                                                                                                                                                                       |                                                                                          |                                                                                                                                                                    |                                                                           |                                        |                                                                                                                                                                                                                                                                                                                     |
|----|--------------------------------------------|-------------------------------------------------------------------------------------------------------------------------------------------------------------------------------------------------------------------------------------------------------|------------------------------------------------------------------------------------------|--------------------------------------------------------------------------------------------------------------------------------------------------------------------|---------------------------------------------------------------------------|----------------------------------------|---------------------------------------------------------------------------------------------------------------------------------------------------------------------------------------------------------------------------------------------------------------------------------------------------------------------|
|    |                                            |                                                                                                                                                                                                                                                       |                                                                                          |                                                                                                                                                                    |                                                                           |                                        | the cohort, annotation by a single radiologist, small dataset                                                                                                                                                                                                                                                       |
| 10 | A. Sarica, Human Brain Mapping, 2017 [112] | To evaluate the potential of a new advanced imaging method to serve as a biomarker for (amyotrophic sclerosis) ALS and use a machine learning technique for ALS diagnosis                                                                             | Classify patients of ALS versus controls (Total 48: 24 ALS, 24 HC)                       | Complete clinical examination by an expert. All patients with ALS met the revised El Escorial criteria for probable, probable laboratory supported or definite ALS | To extract DTI metrics from specific WM tracts                            | Random Forest                          | A: DTI metrics of cerebral penduncle and the corona radiata hold importance in discriminating ALS from controls. Classification accuracy of 80% was obtained. L: small set, no external validation, inconsistency in studies related to clinical metrics and AD, diffusion properties are not biologically specific |
| 11 | H. Wen, Human Brain Mapping, 2017 [113]    | To use diffusion MRI probabilistic tractography and graph theory for investigating the topological organization of whole-brain structural networks in healthy children and drug-naive Tourette Syndrome, and find their relation to clinical features | Classify patients of Tourette Syndrome versus healthy controls (Total: 85, 44 TS, 41 HC) | All the patients met DSM-IV-TR criteria for Tourette Syndrome                                                                                                      | To calculate FA, perform tractography and compute the connectivity matrix | SVM and Multiple Kernel Learning (MKL) | A: Disrupted topological organization of structural networks were found to related to TS and topological features that can help in TS diagnosis were found. Highest classification accuracy (86.47%±3.71 %) and AUC (92.62%±3.35 %) was found using MKL. L: small set, no external validation                       |

|    |                                                        |                                                                                                                                                                                                                        |                                                                                           |                                                                                                                                                 |                                               |         |                                                                                                                                                                                                                                                                                                                             |
|----|--------------------------------------------------------|------------------------------------------------------------------------------------------------------------------------------------------------------------------------------------------------------------------------|-------------------------------------------------------------------------------------------|-------------------------------------------------------------------------------------------------------------------------------------------------|-----------------------------------------------|---------|-----------------------------------------------------------------------------------------------------------------------------------------------------------------------------------------------------------------------------------------------------------------------------------------------------------------------------|
| 12 | J. Del Gaizo, Brian and Behavior, 2017 [114]           | To use machine-learning algorithm to assess the accuracy with which individuals with TLE could be correctly classified as having epilepsy based on voxel- based microstructural abnormalities detected by diffusion MR | Classify temporal lobe epilepsy patients from healthy controls (Total: 68, 32 TLE, 36 HC) | TLE diagnosis was defined in accordance with the criteria proposed by the International League Against Epilepsy (only TLE in left were present) | To extract DTI metrics FA and MD from regions | SVM     | A: In comparison to DTI (accuracy: 0.68), DKI-extracted features (accuracy: 0.82) are better associated with TLE<br>L: small set, no external validation, more studies necessary with consistently misclassified subjects                                                                                                   |
| 13 | J. Underwood, Clinical Infectious Diseases, 2017 [115] | To systematically investigate whether previously proposed subtypes of HIV-associated brain injury were present using a multimodal, machine-learning approach.                                                          | Clustering to discriminate HIV-infected and controls (Total: 213, 134 HIV, 79 HCs)        | 134 HIV-infected participants were recruited to the COBRA study                                                                                 | To extract DTI metrics and perform TBSS       | K-means | A: Despite treatment, cognitive impairment, lower GM volumes and WM volumes were substantially present in HIV-infected population. Two stable clusters (HIV-infected representation: 61.2% and 36.4% resp., odds ratio 2.74, 95% CI: 1.53-4.98) were found<br>L: no external validation, older HIV population, cohort study |
| 14 | P. Fang, Neuroscience Letters, 2017 [116]              | To use machine learning approaches were used to extract the                                                                                                                                                            | Classify patients of mesial temporal lobe epilepsy with                                   | Comprehensive evaluation, including a detailed history, video-EEG                                                                               | To extract DTI metrics and perform            | SVM     | A: Findings suggested left and right mTLE shared a convergent circuit and that                                                                                                                                                                                                                                              |

|    |                                                 |                                                                                                                                                                                                                                                                                               |                                                                                                                                                     |                                                                                                             |                                              |               |                                                                                                                                                                                                                                                                                                                                                                                                                        |
|----|-------------------------------------------------|-----------------------------------------------------------------------------------------------------------------------------------------------------------------------------------------------------------------------------------------------------------------------------------------------|-----------------------------------------------------------------------------------------------------------------------------------------------------|-------------------------------------------------------------------------------------------------------------|----------------------------------------------|---------------|------------------------------------------------------------------------------------------------------------------------------------------------------------------------------------------------------------------------------------------------------------------------------------------------------------------------------------------------------------------------------------------------------------------------|
|    |                                                 | most discriminating connections and to investigate the convergent anatomical network disruptions between left and right mTLE.                                                                                                                                                                 | hippocampal sclerosis and healthy controls (Total: 82, 43 mTLE, 39 HC)                                                                              | telemetry and neuroimaging                                                                                  | tractography                                 |               | helped discriminating left mTLE and controls (generalization rate: 91.7%) and right mTLE and controls (generalization rate: 90.0%)<br>L: small set, no external validation, EEG or clinical data not used for correlation analysis, less powerful features need to be studied                                                                                                                                          |
| 15 | P. M. Ferraro, NeuroImage: Clinical, 2017 [117] | To develop a method for individual identification of motor neuron disease (MND) patients using multi-modal structural MRI data of ALS-specific anatomical regions and to test the validity of such an approach in an independent patient cohort relative to subjects with ALS-mimic disorders | Classify patients of motor neuron diseases, versus mimic diseases versus controls (Total: 265, 123 ALS, 44 PUMN, 20 ALS-mimic disorders, and 78 HC) | ALS diagnosis according to Escorial clinical criteria, ALS-mimic conditions are specific, and clinical PUMN | To extract AD, MD, RD, and FA from WM tracts | Random Forest | A: Multimodal approach using motor cortical and WM alterations in prediction of MND was found effective. Classification accuracy of 0.87 and 0.95 (DTI-based model) and 0.87 and 0.94 (combined model) was found for distinguishing ALS and PUMN patients from mimic syndromes in validation cohort<br>L: small number and heterogeneity of ALS-mimic samples, limitations of Freesurfer (corrections in segmentation) |

|    |                                                                            |                                                                                                                                                                                           |                                                                                                                                             |                                                                                                                                                                                                                                                                                            |                                                                                            |                            |                                                                                                                                                                                                                                                                                                                                        |
|----|----------------------------------------------------------------------------|-------------------------------------------------------------------------------------------------------------------------------------------------------------------------------------------|---------------------------------------------------------------------------------------------------------------------------------------------|--------------------------------------------------------------------------------------------------------------------------------------------------------------------------------------------------------------------------------------------------------------------------------------------|--------------------------------------------------------------------------------------------|----------------------------|----------------------------------------------------------------------------------------------------------------------------------------------------------------------------------------------------------------------------------------------------------------------------------------------------------------------------------------|
|    |                                                                            |                                                                                                                                                                                           |                                                                                                                                             |                                                                                                                                                                                                                                                                                            |                                                                                            |                            | may be necessary), fMRI not incorporated                                                                                                                                                                                                                                                                                               |
| 16 | Y. Garcia-Chimeno, BMC Medical Informatics and Decision Making, 2017 [118] | To automate the diagnosis of patients with migraine through the classification of features obtained from DTI images and psychological tests applied to patients.                          | Classify among chronic, migraine, sporadic migraine patients and healthy controls (Total: 52, 37 patients, 15 HC)                           | Year-long quarterly assessments by a neurology team                                                                                                                                                                                                                                        | To extract FA values                                                                       | SVM, AdaBoost, Naive Bayes | A: Proposed feature selection technique improved the classification accuracy. Highest classification accuracy of 95% was achieved by SVM.<br>L: small set, no external validation and performance may not generalize to external data                                                                                                  |
| 17 | K. Kamiya, Magnetic Resonance Med. Sci., 2016 [119]                        | Examining the performance of a machine learning approach, used in combination with DTI-derived structural connectomes, to determine lateralization of the epileptogenic focus of the TLE. | Classify laterality (left versus right) in Temporal Lobe Epilepsy patients and classify these from controls (Total 58: 44 TLE, 14 controls) | Evaluation of clinical history, seizure semiology and MR imaging, we conducted a comprehensive review of long duration video-EEG recordings or intracranial EEG recordings or positron emission tomography (PET) or single-photon emission computed tomography (SPECT) (36 of 44 patients) | To perform tractography, generate connectivity matrix and extract features from the matrix | SVM                        | A: graph-theoretical measures of DTI structural connectome may help in lateralization of TLE. SVM classifier achieved highest accuracy of 89.7% for right TLE vs. controls<br>L: heterogeneity of patients, effects of drugs taken in patients, DTI streamline count doesn't quantify connection strengths, no external validation set |

|    |                                              |                                                                                                                                                           |                                                                                                                                                                                             |                                                                                                               |                                                       |                     |                                                                                                                                                                                                                                                                                                                                                              |
|----|----------------------------------------------|-----------------------------------------------------------------------------------------------------------------------------------------------------------|---------------------------------------------------------------------------------------------------------------------------------------------------------------------------------------------|---------------------------------------------------------------------------------------------------------------|-------------------------------------------------------|---------------------|--------------------------------------------------------------------------------------------------------------------------------------------------------------------------------------------------------------------------------------------------------------------------------------------------------------------------------------------------------------|
| 18 | H.-J. Chen, Am J Neuroradiology, 2015 [120]  | To explore if DTI features can distinguish cirrhosis as minimal hepatic encephalopathy (MHE) and no hepatic encephalopathy (MHE)                          | Classify patients with cirrhosis as MHE versus NHE (Total: 65, 29 MHE, 36 NHE)                                                                                                              | Battery of Neuropsychological tests                                                                           | To extract DTI metrics FA and MD from WM              | GAMMA, Naive Bayes  | A: Minimal hepatic encephalopathy from absence of encephalopathy can be detected with the help of WM-DTI markers. Highest classification accuracy as 83.1%-92.3% using one of the identified WM regions. L: analysis confined to WM only; a suboptimal DTI sequence with 6 diffusion-encoding gradient directions; only DTI was used, no external validation |
| 19 | B. C. Munsell, NeuroImage, 2015 [121]        | To evaluate accurate surgical outcome estimation could be derived from connectome data alone, and not in combination with other clinical or imaging data, | Classify TLE versus normal controls and Classify treatment outcome (seizure-free versus not free) in patients with epilepsy based on structural connectome data (Total: 118, 70 TLE, 48 HC) | Diagnostic criteria of TLE by ILAE, then at Engel Surgical Outcome scale assessment after one year of surgery | To perform tractography, generate connectivity matrix | SVM                 | A: ML applications on structural connectome can provide expert-level prediction of treatment outcomes. Accuracy for TLE vs. controls was 80% and that for surgical outcomes was 70% L: no external validation                                                                                                                                                |
| 20 | D. Pustina, NeuroImage: Clinical, 2015 [122] | To perform a comprehensive investigation of multimodal data and                                                                                           | Classify laterality (left versus right) in TLE patients (Total: 58, 28                                                                                                                      | Expert board-certified neuroradiologists, epileptologists, and neuropsychologists                             | To extract FA and perform tractography                | Logistic Regression | A: PET (accuracy > 95%) imaging that captured glucose metabolism offered more                                                                                                                                                                                                                                                                                |

|    |                                                                         |                                                                                                                                |                                                                                                                         |                                                                                                                                                                                                                              |                                         |     |                                                                                                                                                                                                                                                         |
|----|-------------------------------------------------------------------------|--------------------------------------------------------------------------------------------------------------------------------|-------------------------------------------------------------------------------------------------------------------------|------------------------------------------------------------------------------------------------------------------------------------------------------------------------------------------------------------------------------|-----------------------------------------|-----|---------------------------------------------------------------------------------------------------------------------------------------------------------------------------------------------------------------------------------------------------------|
|    |                                                                         | develop an automatic classification system for laterality of TLE                                                               | left TLE, 30 right TLE)                                                                                                 | sts, by consensus decision, classified patient neuropathology and seizure type. Intracranial electrodes were implanted to determine the seizure focus through electro-corticography when test information was not sufficient |                                         |     | predictive power compared to DTI (accuracy> 71%) and structural MRI (accuracy> 67%)<br>L: small set, more features from structural MRI and DTI can be used, more heterogeneous samples can be used                                                      |
| 21 | D. Cantor-Rivera, Computerized Medical Imaging and Graphics, 2015 [123] | To improve the detection of TLE using relaxometry and DTI                                                                      | To classify TLE and controls and to classify left and right TLE (Total :36, 9 left TLE, 0 right TLE, 19 controls)       | Lateralizable seizures confirmed by EEG                                                                                                                                                                                      | To extract DTI metrics FA and MD        | SVM | A: For TLE detection, classification accuracy of 88.9% using T1 and MD data was more useful than FA. Accuracy of 100% was obtained using MD for left TLE detection. L: small set, no external validation, sensitivity to the detection of rTLE patients |
| 22 | I. Amarreh, NeuroImage: Clinical, 2014 [124]                            | Investigate SVM as a tool to for classifying seizure outcomes in children with epilepsy (remitted versus persisting seizures). | Classify children and adolescents with active epilepsy, remitted epilepsy, and controls (Total: 49, 20 epilepsy, 29 HC) | Diagnosis of idiopathic epilepsy, remission means no occurrence of epilepsy in 12 months without anti-epileptic drugs                                                                                                        | To extract DTI metrics and perform TBSS | SVM | A: DTI-based FA was able to distinguish active epilepsy patients from remitted epilepsy or control patients with 100% sensitivity and specificity<br>L: small set, heterogeneous seizure syndrome, active epilepsy were on drugs and remitted           |

|    |                                                     |                                                                                                                                                                                                                                                                                 |                                                                                                                                           |                                                                                                            |                                     |                            |                                                                                                                                                                                                                                                                               |
|----|-----------------------------------------------------|---------------------------------------------------------------------------------------------------------------------------------------------------------------------------------------------------------------------------------------------------------------------------------|-------------------------------------------------------------------------------------------------------------------------------------------|------------------------------------------------------------------------------------------------------------|-------------------------------------|----------------------------|-------------------------------------------------------------------------------------------------------------------------------------------------------------------------------------------------------------------------------------------------------------------------------|
|    |                                                     |                                                                                                                                                                                                                                                                                 |                                                                                                                                           |                                                                                                            |                                     |                            | epilepsy were not on drugs, no external validation                                                                                                                                                                                                                            |
| 23 | J. An, Clinical Neuroscience, 2014 [125]            | Use machine learning approaches to investigate the whole-brain white matter changes in mesial Temporal Lobe Epilepsia (mTLE)                                                                                                                                                    | Classify laterality (left versus right) in mTLE patients and classify these from controls (Total: 66, 17 left mTLE, 15 right mTLE, 34 HC) | Medical history, video EEG telemetry, neuroimaging for mTLE; FLAIR signal evaluation in hippocampus for HS | To extract FA from WM tracts        | SVM                        | A: left and right mTLE patients showed decreased FA in specific regions of WM tracts. Highest accuracy was obtained for left mTLE versus controls with accuracy 94.1%, sensitivity 82.4%, and specificity 100%<br>L: small sample size, single-center, no external validation |
| 24 | J.V. Stough, Lecture Notes in Comp. Sc., 2014 [126] | Authors say that this first fully automatic multi-modal thalamus segmentation algorithm, and also the first fully automated thalamic nuclei parcellation—into AN, MD, VNG, PUL, LGN, and MGN—using tensor-based features within the thalamus and cortical connectivity features | Automatic segmentation of thalamus from brain and parts of thalamus nuclei in cerebellar ataxia patients (Total: 12)                      | Manual rater delineated tumor                                                                              | To extract DTI metrics from regions | Hierarchical Random Forest | A: Parcellation of thalamus was accomplished using tissue contrast and diffusion-derived features and mean Dice scores of 0.805 and 0.799 was obtained<br>L: small set, no external validation                                                                                |

|    |                                                 |                                                                                                                                                                  |                                                                                              |                                             |                                                           |               |                                                                                                                                                                                                                                                                                                                                                                                                                                                                                           |
|----|-------------------------------------------------|------------------------------------------------------------------------------------------------------------------------------------------------------------------|----------------------------------------------------------------------------------------------|---------------------------------------------|-----------------------------------------------------------|---------------|-------------------------------------------------------------------------------------------------------------------------------------------------------------------------------------------------------------------------------------------------------------------------------------------------------------------------------------------------------------------------------------------------------------------------------------------------------------------------------------------|
|    |                                                 | derived from tractography.                                                                                                                                       |                                                                                              |                                             |                                                           |               |                                                                                                                                                                                                                                                                                                                                                                                                                                                                                           |
| 25 | M. J. Paldino, NeuroImage: Clinical, 2014 [127] | Measure the independent contribution of the measured diffusion parameters for each tract to the clinical phenotype (language impairment)                         | Classify language phenotype in a pediatric epilepsy cohort (Total: 33)                       | Characterization by a pediatric neurologist | To extract DTI metrics and perform tractography           | Random Forest | A: diffusion metrics derived from specific regions of brain were found to be associated with brain function and classification (sensitivity: 100%, specificity 95.4%) of patient language function was possible with the variables obtained from tractography<br>L: small set of patients selected carefully, importance of variables selected by an algorithm is limited to the set of variables used, functional assessment was limited to a single neurologist, no external validation |
| 26 | E. Ziv, PLOS One, 2013 [128]                    | Utilize data-driven supervised and unsupervised machine learning techniques to study brain connectivity networks and apply those on a dataset of neonatal brains | Classify normal versus abnormal neurological outcomes in neonatal encephalopathy (Total: 24) | Neurologic examination                      | To perform tractography and extract connectivity matrices | SVM           | A: A novel tool was designed for the evaluation of neonates having risk for developing neurological deficits that predicted with an accuracy of $0.79\pm0.04\%$<br>L: the heterogeneity of study cohort                                                                                                                                                                                                                                                                                   |

|    |                                     |                                                                                                                 |                                                                                                        |                                           |                               |     |                                                                                                                                                                                             |
|----|-------------------------------------|-----------------------------------------------------------------------------------------------------------------|--------------------------------------------------------------------------------------------------------|-------------------------------------------|-------------------------------|-----|---------------------------------------------------------------------------------------------------------------------------------------------------------------------------------------------|
|    |                                     |                                                                                                                 |                                                                                                        |                                           |                               |     | –the subjects share the clinical diagnosis of neonatal encephalopathy , but multiple potential etiologies exist for this disorder, the cross-sectional nature of the study, no external set |
| 27 | N. K. Focke, NeuroImage, 2012 [129] | To employ automated MR imaging classification for TLE having unilateral hippocampal sclerosis (HS) and controls | To classify voxels of MR imaging as having left HS, right HS, controls (Total: 60, 38 HS, 22 controls) | Histopathologically confirmed presence of | To extract DTI metrics FA, MD | SVM | A: Automated SVM analysis in mTLE was highly accurate for both binary (accuracies 95-97%) and multiclass classification (accuracy using MD: 93%)<br>L: small set, no external validation    |

**sTable 9 Details of the studies that focused on other miscellaneous Miscellaneous Non-neurological disorders diseases/**  
**Not-Notated**

| <b>Serial Number</b> | <b>First Author, Publication Venue, Year, Reference</b> | <b>Unmet Need</b>                                                                     | <b>Machine Learning Task Performed</b>                                        | <b>Reference Standard for the Disease</b>         | <b>Role of DTI</b> | <b>Machine Learning Model(s) Used</b> | <b>Accomplishments and Limitations (including what authors stated)</b>                                                            |
|----------------------|---------------------------------------------------------|---------------------------------------------------------------------------------------|-------------------------------------------------------------------------------|---------------------------------------------------|--------------------|---------------------------------------|-----------------------------------------------------------------------------------------------------------------------------------|
| 1                    | L. G. Goetschius, NeuroImage, 2019 [130]                | To explore relationships between amygdala and prefrontal cortex (PFC) and use machine | To regress amygdala activation scores from amygdala WM connectivity with five | Task based activation scores extracted using fMRI | tractography       | Ridge Regression                      | A: Significant association between activation scores and amygdala WM connections were found; for happy faces left (MSE: 0.15) and |

|   |                                                   |                                                                                                                                                              |                                                                           |                                                       |                                                             |                                                                                                         |                                                                                                                                                                                                                           |
|---|---------------------------------------------------|--------------------------------------------------------------------------------------------------------------------------------------------------------------|---------------------------------------------------------------------------|-------------------------------------------------------|-------------------------------------------------------------|---------------------------------------------------------------------------------------------------------|---------------------------------------------------------------------------------------------------------------------------------------------------------------------------------------------------------------------------|
|   |                                                   | learning to investigate the association of the amygdala WM connectivity and activation                                                                       | PFCs (Total: 141)                                                         |                                                       |                                                             |                                                                                                         | right (MSE: 0.23) faces was found<br>L: no external validation                                                                                                                                                            |
| 2 | Y. Mu, Journal of Medical Systems, 2019 [131]     | To improve the quality of white matter segmentation in DTI                                                                                                   | Segmentation of white matter (Total: 7000 that has DTI)                   | Details not stated                                    | Chosen imaging modality                                     | FCN based coarse segmentation and two-level optimization using super pixel and mean field approximation | A: A deep-learning based segmentation method is proposed and intersection-over-union (IoU) was 75.2% in this set<br>L: missing details about the self-built dataset                                                       |
| 3 | F. Deng, Brain Structure and Function, 2018 [132] | To better describe the gymnastic training induced neuroplasticity in brain WM tracts                                                                         | To classify gymnasts and controls (Total:27, 13 gymnasts, 14 non-athlete) | History of world-class level gymnastics               | DTI metric extraction, automated fiber tract quantification | logistic regression, SVM                                                                                | A: Fractional anisotropy in deep white matter was able to distinguish between controls and gymnasts with accuracy of 81.48%, sensitivity 84.62%, and specificity 78.57% using SVM<br>L: small set, no external validation |
| 4 | L. Li, Eur Radiology, 2018 [133]                  | To explore the cerebral structural changes related to venous erectile dysfunction (VED) using multimodal MRI and to investigate if the clinical symptoms and | Classify VED from healthy controls (Total: 95, 45 VED, 50 HC)             | Color doppler ultrasound and CT cavernosography exams | To extract DTI metrics and perform TBSS                     | SVM                                                                                                     | A: DTI-derived indices were found to provide discrimination between the VED patients and healthy controls with an accuracy 96.7%, sensitivity 93.3%, and specificity 99.0%<br>L: small set, no external                   |

|   |                                                           |                                                                                                                                                                             |                                                                                            |                               |                                                                                         |                                      |                                                                                                                                                                                                                                                                                                                                                                                   |
|---|-----------------------------------------------------------|-----------------------------------------------------------------------------------------------------------------------------------------------------------------------------|--------------------------------------------------------------------------------------------|-------------------------------|-----------------------------------------------------------------------------------------|--------------------------------------|-----------------------------------------------------------------------------------------------------------------------------------------------------------------------------------------------------------------------------------------------------------------------------------------------------------------------------------------------------------------------------------|
|   |                                                           | durations are associated with cerebral structural alterations                                                                                                               |                                                                                            |                               |                                                                                         |                                      | validation, not a longitudinal design                                                                                                                                                                                                                                                                                                                                             |
| 5 | S. H. Park, Scientific Reports, 2018 [134]                | To investigate if consideration of confounding factors before group analysis removes important information for distinguishing adolescents with and without drinking history | To classify minimal and regular drinkers (Total: 705, 671 minimal and 34 regular drinkers) | Self-reported alcohol history | 112 DTI-derived microstructural values                                                  | Sparse-logistic classification model | A: the approach was found to be impartial to confounding factors, had significance to drinking behaviors and in agreement with literature on alcohol studies, and more accurate after comparison with alternate implementations . The most accurate method included structural MRI and DTI features with an AUC of 83.2% and was not associated with age L:no external validation |
| 6 | Y. Wen, Bio-Medical Materials and Engineering, 2014 [135] | Evaluate tissue segmentation in DTI using multichannel fusion                                                                                                               | Automatic segmentation of grey, white, and cerebrospinal fluid in images (Total: 15)       | Expert segmented ground truth | To extract DTI metrics FA, ADC, Kullback-Leibler Anisotropy (KLA), Axial Diffusion (AD) | Bayesian Decision Theory             | A: Compares favorably with existing methods for segmentation and provides segmentation accuracy of 0.88, 0.85, and 0.76 for WM, GM, and CSF in terms of volume overlap L: Validation on small set, some experimental details missing, unknown nature of cohort                                                                                                                    |
| 7 | X. Hao, Inf. Proc. Med. Imag.                             | A method that jointly solves the tract                                                                                                                                      | Fractional segmentation of white matter tracts                                             | Not stated                    | Estimation of WM tracts                                                                 | MAP, MRF, gradient descent,          | A: Improved segmentation results (lower RMSE < 0.1                                                                                                                                                                                                                                                                                                                                |

|  |                 |                                                                                        |                                  |  |  |                   |                                                                                                                                                  |
|--|-----------------|----------------------------------------------------------------------------------------|----------------------------------|--|--|-------------------|--------------------------------------------------------------------------------------------------------------------------------------------------|
|  | , 2013<br>[136] | segmentation and multi-tensor model estimation problem in low-angular diffusion images | (Total: 1 real data for testing) |  |  | kernel regression | compared to Camino) and diffusion measurement statistics was obtained in presence of crossing tracts and partial voluming<br>L: one real example |
|--|-----------------|----------------------------------------------------------------------------------------|----------------------------------|--|--|-------------------|--------------------------------------------------------------------------------------------------------------------------------------------------|

**sTable 10 Details of the studies that focused on other multiple conditions**

| Serial Number | First Author, Publication Venue, Year, Reference | Unmet Need                   | Machine Learning Task Performed                                                                                         | Reference Standard for the Disease                                        | Role of DTI                          | Machine Learning Model(s) Used | Accomplishments and Limitations (including what authors stated)                                                                                                                                                                                                                                            |
|---------------|--------------------------------------------------|------------------------------|-------------------------------------------------------------------------------------------------------------------------|---------------------------------------------------------------------------|--------------------------------------|--------------------------------|------------------------------------------------------------------------------------------------------------------------------------------------------------------------------------------------------------------------------------------------------------------------------------------------------------|
| 1             | E. Aliotta, Medical Physics, 2019 [137]          | To reconstruct DTI using ANN | To reconstruct MD and FA maps of DTI using ANN (Total: 22, training set: 10 healthy patients, Testing: 12 GBM patients) | Linear least square-based fitting to generate ground truth FA and MD maps | Imaging modality chosen for the task | ANN                            | A: Improved DTI reconstruction AUC (0.926), precision, and tumor delineation performance in GBM was obtained and reconstruction was possible from only three diffusion-encoding directions<br>L: small set, downward bias for high FA values, fixed diffusion-encoding gradient directions set and b-value |
| 2             | T. Kuhn, Human Brain                             | Investigating the predicted  | Regress age of healthy humans from                                                                                      | Clinical (healthy                                                         | To extract DTI                       | SVR (predict                   | A: Study found                                                                                                                                                                                                                                                                                             |

|   |                                          |                                                                                                  |                                                                                                     |                                                                                                                           |                                 |                     |                                                                                                                                                                                                                                                                                                                                                                                                                                                                                                                                                                             |
|---|------------------------------------------|--------------------------------------------------------------------------------------------------|-----------------------------------------------------------------------------------------------------|---------------------------------------------------------------------------------------------------------------------------|---------------------------------|---------------------|-----------------------------------------------------------------------------------------------------------------------------------------------------------------------------------------------------------------------------------------------------------------------------------------------------------------------------------------------------------------------------------------------------------------------------------------------------------------------------------------------------------------------------------------------------------------------------|
|   | Mapping, 2018 [138]                      | brain white matter age different in WM microstructure using DTI metrics of white matter patency. | imaging and predict brain age gap in HIV+ and HIV- patients (Total: 869, 765 training, 104 testing) | status from ongoing studies in training set) and Self-reported (self-reported nadir CD41 and lifetime highest viral load) | metrics from ROIs, perform TBSS | chronological age)  | augmented WM aging in HIV patients. Predicted brain age gap was significantly higher in HIV+ group and negatively correlated ( $r = -0.26$ ) with cognitive function<br>L: Cross-section study design, SVR modeling using DTI was had more error compared to that using T1, WM lesions were not controlled for demographic differences in train and test set, exclusion of participants with substance use disorders and Axis I diagnoses, presence of pre-HAART and post HAART era patients, the DTI-based WM metrics were extracted from the entire white matter skeleton |
| 3 | G. Ball, Human Brain Mapping, 2017 [139] | To apply an unsupervised and data-driven                                                         | Clustering sub-networks in brain in healthy and ASD separately (Total:                              | High-functioning children with ASD                                                                                        | To extract DTI metrics          | ARD-PNMF (automatic | A: Probable long-term effects of changes to the                                                                                                                                                                                                                                                                                                                                                                                                                                                                                                                             |

|   |                                       |                                                                                                                                                                  |                                                                                       |                                                                                                                                                 |                                                                                              |                                                                                |                                                                                                                                                                                                                                                                                                                                       |
|---|---------------------------------------|------------------------------------------------------------------------------------------------------------------------------------------------------------------|---------------------------------------------------------------------------------------|-------------------------------------------------------------------------------------------------------------------------------------------------|----------------------------------------------------------------------------------------------|--------------------------------------------------------------------------------|---------------------------------------------------------------------------------------------------------------------------------------------------------------------------------------------------------------------------------------------------------------------------------------------------------------------------------------|
|   |                                       | approach for modelling complex networks derived from whole-brain tractography as a set of components, or sub-networks, that vary together across the population. | 290, expt. 1: 196 healthy, expt 2: 51 ASD, 43 controls)                               | had a prior clinical diagnosis of autism based on criteria from the DSM-IV with additional confirmation; Healthy patients from a public dataset |                                                                                              | relevance determination based on projective non-negative matrix factorization) | developmental trajectories of specific cortical subnetworks were found. Reliability assessment was performed.<br><br>L: no external validation; log-transformation of streamlines may be an issue; only high-functioning ASD were included as specific alterations in brain morphology are not present in all ASD subtypes            |
| 4 | J. D. Medaglia, Neurology, 2017 [140] | To apply network-analytic techniques to multimodal neuroimaging data to differentiate pathological drivers of cortico-basal syndrome (CBS), AD, and HC           | Classify AD, non-AD in the context of CBS, and HC (Total 80: AD 21, non-AD 19, HC 40) | Clinically diagnosed CBS and AD or non-AD pathology was confirmed by autopsy, genetic or CSF findings                                           | To extract features values from connectivity matrix obtained using gray matter tract regions | SVM                                                                            | A: Better performance (85% sensitivity, 84% specificity) in classification of pathologic sources of corticobasal syndrome was possible using graph theoretical statistics derived from patterns of WM network organization in association cortex than by regional gray matter density alone.<br>L: small set, no external validation, |

|   |                                                  |                                                                                                                                             |                                                                                                                                                                       |                                                                                                            |                                                                                       |                                                                                  |                                                                                                                                                                                                                                                                                                                                                     |
|---|--------------------------------------------------|---------------------------------------------------------------------------------------------------------------------------------------------|-----------------------------------------------------------------------------------------------------------------------------------------------------------------------|------------------------------------------------------------------------------------------------------------|---------------------------------------------------------------------------------------|----------------------------------------------------------------------------------|-----------------------------------------------------------------------------------------------------------------------------------------------------------------------------------------------------------------------------------------------------------------------------------------------------------------------------------------------------|
|   |                                                  |                                                                                                                                             |                                                                                                                                                                       |                                                                                                            |                                                                                       |                                                                                  | commonly applied statistics were used, only DTI tractography                                                                                                                                                                                                                                                                                        |
| 5 | A. Besga, Current Alzheimer Research, 2016 [141] | To study identify the localization of white matter effects correlated with biomarkers by applying an eigenanatomy-based feature extraction. | Classify patients of Alzheimer's Disease versus Late Onset Bipolar Disorder (Total: 78, 35 AD, 24 BD, 19 HC)                                                          | BD group fulfills the DSM IV criteria and the AD group fulfills the NINCDS-ADRDA criteria for probable AD. | FA extraction                                                                         | SVM                                                                              | A: Eigenanatomy-based features of FA correlated to plasma biomarkers were able to distinguish between LOBD and AD. Best classification performance (accuracy 85%, F-score 86%, sensitivity, and specificity 87%) was obtained by a biomarker of oxidative stress.<br>L: no external validation, diverse number of samples of AD, BD, and HC present |
| 6 | A. Yendiki, NeuroImage, 2016 [142]               | To reconstruct WM pathways in brain using data from several time points                                                                     | Reconstruction of white matter pathways (33 healthy subjects for training, 9 healthy for test - retest, 46 subjects of Huntington's disease for sensitivity analysis) | Tracks labelled by neuroanatomy experts                                                                    | Longitudinal diffusion information used in the process of reconstruction of WM tracts | Proposed approach to estimate probability of distribution of a subject's pathway | A: Enhanced reliability in reconstruction in WM pathways (average error was 5% in healthy patients, 22.3% of 18 pathway positions showed changes for Huntington's disease) was obtained with constructing                                                                                                                                           |

|   |                                         |                                                                                                                                                                                                          |                                                                                                                                                                                                                             |                                                                                                                                                                                                                                 |               |             |                                                                                                                                                                                                                                                                                           |
|---|-----------------------------------------|----------------------------------------------------------------------------------------------------------------------------------------------------------------------------------------------------------|-----------------------------------------------------------------------------------------------------------------------------------------------------------------------------------------------------------------------------|---------------------------------------------------------------------------------------------------------------------------------------------------------------------------------------------------------------------------------|---------------|-------------|-------------------------------------------------------------------------------------------------------------------------------------------------------------------------------------------------------------------------------------------------------------------------------------------|
|   |                                         |                                                                                                                                                                                                          |                                                                                                                                                                                                                             |                                                                                                                                                                                                                                 |               |             | white-matter pathways jointly using the longitudinal data compared to the cross-sectional data using the fully automated method.<br>L: Small set                                                                                                                                          |
| 7 | C. J. Lin, PloS One, 2014 [143]         | To determine whether connectivity markers may be used to aid early diagnosis of MCI/VCIND and identify the most appropriate patients for revascularization at pre-symptomatic stages of carotid stenosis | Classify mild cognitive impairment or severe dizziness in pre-symptomatic carotid stenosis (Total 60, 30 with findings 30 HC)                                                                                               | extracranial internal carotid artery by ultrasound; cut-off value of delayed verbal recall or DHI scores as 1.5 SD below the mean of healthy control group was used to classify individuals with MCI/VCIND or severe dizziness. | To extract FA | SVM         | A: Multivariate classification model achieved more 90% accuracy in predicting MCI or severe dizziness<br>L: Brain perfusion was not evaluated and shorter TR was used for improved SNR. Fiber tractography was not done, a cross-sectional case-control study; no external validation set |
| 8 | N. Adluru, Neuroinformatics. 2013 [144] | Understand the relationship of voxel-based morphometry and multi-voxel pattern analysis in neuroimaging and unify these with VBM and MVPA by using penalized likelihood modeling (PLM)                   | Classify ASD and TDs (Total 155: 55 TD, 99 ASD)<br>Regress the Social Reciprocity/Responsiveness Scale scores in long term meditation (LTM) practitioners and meditation naive practitioners/MNP (Total 49: 23 MNP, 26 LTM) | ASD diagnosis and self-reported retreat hours                                                                                                                                                                                   | To derive FA  | SVM and SVR | A: Unification of VBM and MVPA and utilization of novel metrics for evaluation. Highest accuracy of 72.58% for ASD detection, lowest MSE of 0.55 for meditation<br>L: small set, no external validation                                                                                   |

|    |                                                                  |                                                                                                                                                                                                              |                                                                                                                                                                                         |                                                   |                                                 |                                      |                                                                                                                                                                                                                                                                                                                                                                   |
|----|------------------------------------------------------------------|--------------------------------------------------------------------------------------------------------------------------------------------------------------------------------------------------------------|-----------------------------------------------------------------------------------------------------------------------------------------------------------------------------------------|---------------------------------------------------|-------------------------------------------------|--------------------------------------|-------------------------------------------------------------------------------------------------------------------------------------------------------------------------------------------------------------------------------------------------------------------------------------------------------------------------------------------------------------------|
| 9  | C.-Y. Chu, Computerized Medical Imaging and Graphics, 2015 [145] | To overcome the local uncertainty in the estimation of intravoxel fiber orientations by using the orientation information of neighboring fibers in the process of the streamline tracking                    | Reconstructing multifiber pathways in human brain for fiber tracking (Total 20 real: 10 normal, 10 SZ)                                                                                  | SZ diagnosis                                      | To estimate tensor and perform tractography     | Bundle Constrained Streamline        | A: Outperforms (average spatial metric 2.72 mm) the existing techniques to allow regular pathways to be reconstructed.<br>L: Model works on the assumptions that fiber bundles are locally smooth and can be affected by trauma/pathology                                                                                                                         |
| 10 | T. Zhang, Medical Image Analysis, 2013, [146]                    | Few studies have investigated whether DTI derived connectional features and T1-weighted MRI derived anatomical features can be integrated to improve the performance of predicting functional cortical ROIs. | Localization of cortical region-of-interest from task-based fMRI using DTI and T1-weighted MRI data (Total: 35, Dataset 1 -11 healthy, Dataset 2 -17 healthy, Dataset 3 – 7 from ADNI2) | Algorithmically detected ROI from task-based fMRI | To perform tractography and tissue segmentation | Generalized Multiple Kernel Learning | A: ROI localization models were evaluated on independent datasets. Prediction errors were lower (max: 8.08 mm) compared to four other methods<br>L: Focusses on most consistent ROIs, but other potentially important factors such as descriptive power of features, ROI location variability across subjects and ROI size are not taken into consideration; peak |

|    |                                                  |                                                                                                                                                                                                 |                                                                                                                                                                                                                      |                                                              |                                                           |                          |                                                                                                                                                                                                                                                    |
|----|--------------------------------------------------|-------------------------------------------------------------------------------------------------------------------------------------------------------------------------------------------------|----------------------------------------------------------------------------------------------------------------------------------------------------------------------------------------------------------------------|--------------------------------------------------------------|-----------------------------------------------------------|--------------------------|----------------------------------------------------------------------------------------------------------------------------------------------------------------------------------------------------------------------------------------------------|
|    |                                                  |                                                                                                                                                                                                 |                                                                                                                                                                                                                      |                                                              |                                                           |                          | activations detected from fMRI data may be shifted by some factors; applicable to cortical ROIs only                                                                                                                                               |
| 11 | Y. Ghanbari, Inf Process Med Imaging. 2013 [147] | Decomposition of connectivity matrices into interpretable basis components to obtain a low dimensional representation of the population                                                         | Clustering DTI connectivity matrices analyzing children with ASD and TDs and analyzing gender differences in different cohorts (Dataset 1: 83 children, 24 ASD and 59 typically developing, Dataset 2: 595 subjects) | Not stated                                                   | To perform tractography and extract connectivity matrices | NMF with graph embedding | A: Clustering methodology works on two diverse datasets based on t-tests conducted on the coefficients of the components.<br>L: no external validation                                                                                             |
| 12 | A. Besga, Neuroscience Letters, 2012 [148]       | Using Computer aided diagnosis (CAD) systems to improve the prediction accuracy in the diagnosis of Alzheimer's complementing the neuropsychological assessments performed by expert clinicians | Classify among AD, BD, and healthy controls (Total: 57, 20 AD, 12 BD, 25 HC)                                                                                                                                         | NINDS-ADRDA criteria for probable AD, DSM-IV criteria for BD | To extract FA                                             | SVM                      | A: Major tracts were identified were shown to be affected in AD. 100% accuracy for AD vs. BD and AD vs. HC using FA.<br>L: no external validation cross-sectional study with small number of participants, effect of medication was not considered |

#### References:

- [1] A. Ciritsis, A. Boss, and C. Rossi, "Automated pixel-wise brain tissue segmentation of diffusion-weighted images via machine learning," *NMR Biomed.*, vol. 31, no. 7, p. e3931, Jul. 2018.
- [2] N. S. Gorbach, M. Tittgemeyer, and J. M. Buhmann, "Pipeline validation for connectivity-based cortex parcellation," *Neuroimage*, vol. 181, pp. 219–234, 2018.
- [3] S. Genon *et al.*, "The heterogeneity of the left dorsal premotor cortex evidenced by multimodal connectivity-based parcellation and functional characterization," *Neuroimage*, 2018.
- [4] T. Fuchigami, Y. Shikauchi, K. Nakae, M. Shikauchi, T. Ogawa, and S. Ishii, "Zero-shot fMRI decoding with three-

- dimensional registration based on diffusion tensor imaging,” *Sci. Rep.*, vol. 8, no. 1, pp. 1–11, Dec. 2018.
- [5] J. Kawahara *et al.*, “BrainNetCNN: Convolutional neural networks for brain networks; towards predicting neurodevelopment,” *Neuroimage*, vol. 146, pp. 1038–1049, Feb. 2017.
- [6] L. Lin, C. Jin, Z. Fu, B. Zhang, G. Bin, and S. Wu, “Predicting healthy older adult’s brain age based on structural connectivity networks using artificial neural networks,” *Comput. Methods Programs Biomed.*, vol. 125, pp. 8–17, Mar. 2016.
- [7] D. Wang *et al.*, “Human connectome module pattern detection using a new multi-graph MinMax cut model,” in *Lecture Notes in Computer Science (including subseries Lecture Notes in Artificial Intelligence and Lecture Notes in Bioinformatics)*, 2014.
- [8] H. Ullman, R. Almeida, and T. Klingberg, “Structural maturation and brain activity predict future working memory capacity during childhood development,” *J. Neurosci.*, vol. 34, no. 5, pp. 1592–8, Jan. 2014.
- [9] B. Mwangi, K. M. Hasan, and J. C. Soares, “Prediction of individual subject’s age across the human lifespan using diffusion tensor imaging: a machine learning approach,” *Neuroimage*, vol. 75, pp. 58–67, Jul. 2013.
- [10] R. Yun, C. C. Lin, S. Wu, C. C. Huang, C. P. Lin, and Y. P. Chao, “A prediction model for cognitive performance in health ageing using diffusion tensor imaging with graph theory,” in *Proceedings of the Annual International Conference of the IEEE Engineering in Medicine and Biology Society, EMBS*, 2013.
- [11] Y. Wen, L. He, K. M. von Deneen, and Y. Lu, “Brain tissue classification based on DTI using an improved fuzzy C-means algorithm with spatial constraints,” *Magn. Reson. Imaging*, vol. 31, no. 9, pp. 1623–30, Nov. 2013.
- [12] I. I. Maximov, E. Farrher, F. Grinberg, and N. J. Shah, “Spatially variable Rician noise in magnetic resonance imaging,” *Med. Image Anal.*, vol. 16, no. 2, pp. 536–48, Feb. 2012.
- [13] Z. Hua, D. B. Dunson, J. H. Gilmore, M. A. Styner, and H. Zhu, “Semiparametric Bayesian local functional models for diffusion tensor tract statistics,” *Neuroimage*, vol. 63, no. 1, pp. 460–74, Oct. 2012.
- [14] A. Crippa, L. Cerliani, L. Nanetti, and J. B. T. M. Roerdink, “Heuristics for connectivity-based brain parcellation of SMA/pre-SMA through force-directed graph layout,” *Neuroimage*, 2011.
- [15] E. C. Robinson, A. Hammers, A. Ericsson, A. David Edwards, and D. Rueckert, “Identifying population differences in whole-brain structural networks: A machine learning approach,” *Neuroimage*, vol. 50, pp. 910–919, 2010.
- [16] H. Zhuang *et al.*, “Multimodal classification of drug-naïve first-episode schizophrenia combining anatomical, diffusion and resting state functional resonance imaging,” *Neurosci. Lett.*, vol. 705, pp. 87–93, 2019.
- [17] X. Wang *et al.*, “Rehabilitative compensatory mechanism of hierarchical subnetworks in major depressive disorder: A longitudinal study across multi-sites,” *Eur. Psychiatry*, vol. 58, pp. 54–62, 2019.
- [18] Y. Deng *et al.*, “Tractography-based classification in distinguishing patients with first-episode schizophrenia from healthy individuals,” *Prog. Neuro-Psychopharmacology Biol. Psychiatry*, vol. 88, pp. 66–73, Jan. 2019.
- [19] D. Alnæs *et al.*, “Association of heritable cognitive ability and psychopathology with white matter properties in children and adolescents,” *JAMA Psychiatry*, vol. 75, no. 3, pp. 287–295, Mar. 2018.
- [20] F. Deng *et al.*, “Abnormal segments of right uncinate fasciculus and left anterior thalamic radiation in major and bipolar depression,” *Prog. Neuro-Psychopharmacology Biol. Psychiatry*, 2018.
- [21] P. Mikolas *et al.*, “Machine learning classification of first-episode schizophrenia spectrum disorders and controls using whole brain white matter fractional anisotropy,” *BMC Psychiatry*, 2018.
- [22] S. H. Chu, C. Lenglet, M. W. Schreiner, B. Klimes-Dougan, K. Cullen, and K. K. Parhi, “Anatomical Biomarkers for Adolescent Major Depressive Disorder from Diffusion Weighted Imaging using SVM Classifier,” in *Proceedings of the Annual International Conference of the IEEE Engineering in Medicine and Biology Society, EMBS*, 2018, vol. 2018-July, pp. 2740–2743.
- [23] S. H. Chu, C. Lenglet, M. W. Schreiner, B. Klimes-Dougan, K. Cullen, and K. K. Parhi, “Classifying Treated vs. Untreated MDD Adolescents from Anatomical Connectivity using Nonlinear SVM,” in *Proceedings of the Annual International Conference of the IEEE Engineering in Medicine and Biology Society, EMBS*, 2018, vol. 2018-July, pp. 1–4.
- [24] M.-J. Wu *et al.*, “Identification and individualized prediction of clinical phenotypes in bipolar disorders using neurocognitive data, neuroimaging scans and machine learning,” *Neuroimage*, vol. 145, no. Pt B, pp. 254–264, Jan. 2017.
- [25] T. M. Chaim-Avancini *et al.*, “Neurobiological support to the diagnosis of ADHD in stimulant-naïve adults: pattern recognition analyses of MRI data,” *Acta Psychiatr. Scand.*, vol. 136, no. 6, pp. 623–636, Dec. 2017.
- [26] G. Pfuhl *et al.*, “Preserved white matter microstructure in young patients with anorexia nervosa?,” *Hum. Brain Mapp.*, vol. 37, no. 11, pp. 4069–4083, Nov. 2016.
- [27] K. Bi, L. Hua, M. Wei, J. Qin, Z. Yao, and Q. Lu, “Dynamic functional-structural coupling within acute functional state change phases: Evidence from a depression recognition study,” *J. Affect. Disord.*, vol. 191, pp. 145–155, 2016.
- [28] S. Mas *et al.*, “Integrating genetic, neuropsychological and neuroimaging data to model early-onset obsessive compulsive disorder severity,” *PLoS One*, vol. 11, no. 4, 2016.
- [29] B. Mwangi *et al.*, “Predictive classification of pediatric bipolar disorder using atlas-based diffusion weighted imaging and support vector machines,” *Psychiatry Res.*, vol. 234, no. 2, pp. 265–271, Nov. 2015.
- [30] D. Peruzzo *et al.*, “Classification of first-episode psychosis: a multi-modal multi-feature approach integrating structural and diffusion imaging,” *J. Neural Transm.*, vol. 122, pp. 897–905, 2015.
- [31] I. Zwir *et al.*, “Decomposition of brain diffusion imaging data uncovers latent schizophrenias with distinct patterns of

- white matter anisotropy,” *Neuroimage*, 2015.
- [32] J. Qin *et al.*, “Altered anatomical patterns of depression in relation to antidepressant treatment: Evidence from a pattern recognition analysis on the topological organization of brain networks,” *J. Affect. Disord.*, vol. 180, pp. 129–137, 2015.
  - [33] Y. Jin *et al.*, “Identification of infants at high-risk for autism spectrum disorder using multiparameter multiscale white matter connectivity networks,” *Hum. Brain Mapp.*, vol. 36, no. 12, pp. 4880–96, Dec. 2015.
  - [34] F. Li *et al.*, “Multivariate pattern analysis of DTI reveals differential white matter in individuals with obsessive-compulsive disorder,” *Hum. Brain Mapp.*, vol. 35, no. 6, pp. 2643–51, Jun. 2014.
  - [35] J. Qin *et al.*, “Abnormal hubs of white matter networks in the frontal-parieto circuit contribute to depression discrimination via pattern classification,” *Magn. Reson. Imaging*, 2014.
  - [36] W. Pettersson-Yeo *et al.*, “Using genetic, cognitive and multi-modal neuroimaging data to identify ultra-high-risk and first-episode psychosis at the individual level,” *Psychol. Med.*, 2013.
  - [37] M. Ingalhalikar, R. Verma, T. P. L. Roberts, R. Gur, A. R. Smith, and L. Bloy, “Identifying Sub-Populations via Unsupervised Cluster Analysis on Multi-Edge Similarity Graphs,” 2012.
  - [38] P. Fang *et al.*, “Increased cortical-limbic anatomical network connectivity in major depression revealed by diffusion tensor imaging,” *PLoS One*, vol. 7, no. 9, p. e45972, Sep. 2012.
  - [39] A. L. Fouque *et al.*, “Voxelwise multivariate statistics and brain-wide machine learning using the full diffusion tensor,” in *Lecture Notes in Computer Science (including subseries Lecture Notes in Artificial Intelligence and Lecture Notes in Bioinformatics)*, 2011.
  - [40] M. Ingalhalikar, D. Parker, L. Bloy, T. P. L. Roberts, and R. Verma, “Diffusion based abnormality markers of pathology: toward learned diagnostic prediction of ASD,” *Neuroimage*, vol. 57, no. 3, pp. 918–27, Aug. 2011.
  - [41] A. Vamvakas *et al.*, “Imaging biomarker analysis of advanced multiparametric MRI for glioma grading,” *Phys. Medica*, vol. 60, pp. 188–198, 2019.
  - [42] L. S. Hu *et al.*, “Accurate Patient-specific Machine Learning Models Of Glioblastoma Invasion Using Transfer Learning HHS Public Access,” *AJNR Am J Neuroradiol*, vol. 40, no. 3, pp. 418–425, 2019.
  - [43] S. Shrot, M. Salhov, N. Dvorski, E. Konen, A. Averbuch, and C. Hoffmann, “Application of MR morphologic, diffusion tensor, and perfusion imaging in the classification of brain tumors using machine learning scheme,” *Neuroradiology*, vol. 61, no. 7, pp. 757–765, 2019.
  - [44] X. Leng *et al.*, “Application of a machine learning method to whole brain white matter injury after radiotherapy for nasopharyngeal carcinoma,” *Cancer Imaging*, vol. 19, no. 1, Mar. 2019.
  - [45] F. Citak-Er, Z. Firat, I. Kovanlikaya, U. Ture, and E. Ozturk-Isik, “Machine-learning in grading of gliomas based on multi-parametric magnetic resonance imaging at 3T,” *Comput. Biol. Med.*, vol. 99, no. 8, pp. 154–160, 2018.
  - [46] H. Akbari *et al.*, “In vivo evaluation of EGFRvIII mutation in primary glioblastoma patients via complex multiparametric MRI signature,” *Neuro. Oncol.*, vol. 20, no. 8, pp. 1068–1079, 2018.
  - [47] L. Chen *et al.*, “Multi-Label Nonlinear Matrix Completion With Transductive Multi-Task Feature Selection for Joint MGMT and IDH1 Status Prediction of Patient With High-Grade Gliomas,” *IEEE Trans. Med. Imaging*, vol. 37, no. 8, pp. 1775–1787, 2018.
  - [48] M. Soltaninejad *et al.*, “Supervised learning based multimodal MRI brain tumour segmentation using texture features from supervoxels,” *Comput. Methods Programs Biomed.*, vol. 157, pp. 69–84, Apr. 2018.
  - [49] L. Chen *et al.*, “Multi-label Inductive Matrix Completion for Joint MGMT and IDH1 Status Prediction for Glioma Patients,” *Med. Image Comput. Comput. Assist. Interv.*, vol. 10434, pp. 450–458, Sep. 2017.
  - [50] P. Eichinger *et al.*, “Diffusion tensor image features predict IDH genotype in newly diagnosed WHO grade II/III gliomas,” *Sci. Rep.*, vol. 7, no. 1, 2017.
  - [51] L. Liu, H. Zhang, I. Rekik, X. Chen, Q. Wang, and D. Shen, “Outcome prediction for patient with high-grade gliomas from brain functional and structural networks,” in *Lecture Notes in Computer Science (including subseries Lecture Notes in Artificial Intelligence and Lecture Notes in Bioinformatics)*, 2016.
  - [52] X. Qian, H. Tan, J. Zhang, W. Zhao, M. D. Chan, and X. Zhou, “Stratification of pseudoprogression and true progression of glioblastoma multiforme based on longitudinal diffusion tensor imaging without segmentation,” *Med. Phys.*, vol. 43, no. 11, pp. 5889–5902, Nov. 2016.
  - [53] J. Zhang *et al.*, “Pseudo progression identification of glioblastoma with dictionary learning,” *Comput. Biol. Med.*, vol. 73, pp. 94–101, Jun. 2016.
  - [54] H. Akbari *et al.*, “Imaging Surrogates of Infiltration Obtained Via Multiparametric Imaging Pattern Analysis Predict Subsequent Location of Recurrence of Glioblastoma,” *Neurosurgery*, vol. 78, no. 4, pp. 572–80, Apr. 2016.
  - [55] L. S. Hu *et al.*, “Multi-Parametric MRI and Texture Analysis to Visualize Spatial Histologic Heterogeneity and Tumor Extent in Glioblastoma,” *PLoS One*, vol. 10, no. 11, p. e0141506, Nov. 2015.
  - [56] S. Shibata *et al.*, “Voxel-based clustered imaging by multiparameter diffusion tensor images for glioma grading,” *NeuroImage Clin.*, 2014.
  - [57] G. Yang, T. L. Jones, T. R. Barrick, and F. A. Howe, “Discrimination between glioblastoma multiforme and solitary metastasis using morphological features derived from the p: Q tensor decomposition of diffusion tensor imaging,” *NMR Biomed.*, 2014.
  - [58] P. Svolos *et al.*, “Investigating brain tumor differentiation with diffusion and perfusion metrics at 3T MRI using pattern recognition techniques,” *Magn. Reson. Imaging*, vol. 31, no. 9, pp. 1567–1577, 2013.
  - [59] P. Svolos *et al.*, “Classification methods for the differentiation of atypical meningiomas using diffusion and perfusion

- techniques at 3-T MRI,” *Clin. Imaging*, vol. 37, no. 5, pp. 856–64, Sep. 2013.
- [60] V. M. Vergara, A. R. Mayer, E. Damaraju, K. A. Kiehl, and V. Calhoun, “Detection of Mild Traumatic Brain Injury by Machine Learning Classification Using Resting State Functional Network Connectivity and Fractional Anisotropy,” *J. Neurotrauma*, vol. 34, no. 5, pp. 1045–1053, Sep. 2016.
- [61] Z. S. Zheng, N. Reggente, E. Lutkenhoff, A. M. Owen, and M. M. Monti, “Disentangling disorders of consciousness: Insights from diffusion tensor imaging and machine learning,” *Hum. Brain Mapp.*, vol. 38, no. 1, pp. 431–443, Jan. 2017.
- [62] R. Goswami *et al.*, “Frontotemporal correlates of impulsivity and machine learning in retired professional athletes with a history of multiple concussions,” *Brain Struct. Funct.*, vol. 221, no. 4, pp. 1911–1925, 2016.
- [63] E. D. Fagerholm, P. J. Hellyer, G. Scott, R. Leech, and D. J. Sharp, “Disconnection of network hubs and cognitive impairment after traumatic brain injury,” *Brain*, vol. 138, no. Pt 6, pp. 1696–709, Jun. 2015.
- [64] P. J. Hellyer, R. Leech, T. E. Ham, V. Bonnelle, and D. J. Sharp, “Individual prediction of white matter injury following traumatic brain injury,” *Ann. Neurol.*, vol. 73, no. 4, pp. 489–499, 2013.
- [65] A. Wada *et al.*, “Differentiating Alzheimer’s disease from dementia with lewy bodies using a deep learning technique based on structural brain connectivity,” *Magn. Reson. Med. Sci.*, vol. 18, no. 3, pp. 219–224, 2019.
- [66] M. J. Knight, A. Wearn, E. Coulthard, and R. A. Kauppinen, “T2 Relaxometry and Diffusion Tensor Indices of the Hippocampus and Entorhinal Cortex Improve Sensitivity and Specificity of MRI to Detect Amnesic Mild Cognitive Impairment and Alzheimer’s Disease Dementia,” *J. Magn. Reson. Imaging*, vol. 49, no. 2, pp. 445–455, Feb. 2019.
- [67] M. J. R. J. Bouts *et al.*, “Detection of mild cognitive impairment in a community-dwelling population using quantitative, multiparametric MRI-based classification,” *Hum. Brain Mapp.*, vol. 40, no. 9, pp. 2711–2722, Jun. 2019.
- [68] G. W. Eldeeb, N. Zayed, and I. A. Yassine, “Alzheimer’s Disease Classification Using Bag-Of-Words Based on Visual Pattern of Diffusion Anisotropy for DTI Imaging,” in *Proceedings of the Annual International Conference of the IEEE Engineering in Medicine and Biology Society, EMBS*, 2018, vol. 2018-July, pp. 57–60.
- [69] R. A. Feis *et al.*, “Single-subject classification of presymptomatic frontotemporal dementia mutation carriers using multimodal MRI,” *NeuroImage Clin.*, vol. 20, pp. 188–196, 2018.
- [70] E. E. Bron *et al.*, “Multiparametric computer-aided differential diagnosis of Alzheimer’s disease and frontotemporal dementia using structural and advanced MRI,” *Eur. Radiol.*, vol. 27, no. 8, pp. 3372–3382, Aug. 2017.
- [71] T. M. Schouten *et al.*, “Individual classification of Alzheimer’s disease with diffusion magnetic resonance imaging,” *Neuroimage*, vol. 152, pp. 476–481, 2017.
- [72] T. Maggipinto *et al.*, “DTI measurements for Alzheimer’s classification,” *Phys. Med. Biol.*, vol. 62, no. 6, pp. 2361–2375, Mar. 2017.
- [73] Y. Chen *et al.*, “Automated detection of pathologic white matter alterations in Alzheimer’s disease using combined diffusivity and kurtosis method,” *Psychiatry Res. Neuroimaging*, vol. 264, pp. 35–45, Jun. 2017.
- [74] S. Ciulli *et al.*, “Prediction of Impaired Performance in Trail Making Test in MCI Patients with Small Vessel Disease Using DTI Data,” *IEEE J. Biomed. Heal. Informatics*, vol. 20, no. 4, pp. 1026–1033, 2016.
- [75] M. Dyrba, M. Grothe, T. Kirste, and S. J. Teipel, “Multimodal analysis of functional and structural disconnection in Alzheimer’s disease using multiple kernel SVM,” *Hum. Brain Mapp.*, vol. 36, no. 6, pp. 2118–2131, 2015.
- [76] M. Dyrba *et al.*, “Predicting Prodromal Alzheimer’s Disease in Subjects with Mild Cognitive Impairment Using Machine Learning Classification of Multimodal Multicenter Diffusion-Tensor and Magnetic Resonance Imaging Data,” *J. Neuroimaging*, vol. 25, no. 5, pp. 738–747, 2015.
- [77] S. Diciotti *et al.*, “Multimodal MRI classification in vascular mild cognitive impairment,” in *Proceedings of the Annual International Conference of the IEEE Engineering in Medicine and Biology Society, EMBS*, 2015, vol. 2015-Novem, pp. 4278–4281.
- [78] Y. Xie *et al.*, “Identification of Amnesic Mild Cognitive Impairment Using Multi-Modal Brain Features: A Combined Structural MRI and Diffusion Tensor Imaging Study,” *J. Alzheimer’s Dis.*, vol. 47, no. 2, pp. 509–522, Jul. 2015.
- [79] D. Zhu *et al.*, “Connectome-scale assessments of structural and functional connectivity in MCI,” *Hum. Brain Mapp.*, vol. 35, no. 7, pp. 2911–23, Jul. 2014.
- [80] J. A. Pineda-Pardo *et al.*, “Guiding functional connectivity estimation by structural connectivity in MEG: An application to discrimination of conditions of mild cognitive impairment,” *Neuroimage*, vol. 101, pp. 765–777, 2014.
- [81] M. Li, Y. Qin, F. Gao, W. Zhu, and X. He, “Discriminative analysis of multivariate features from structural MRI and diffusion tensor images,” *Magn. Reson. Imaging*, vol. 32, no. 8, pp. 1043–51, Oct. 2014.
- [82] M. Dyrba, M. Ewers, M. Wegrzyn, I. Kilimann, and C. Plant, “Robust Automated Detection of Microstructural White Matter Degeneration in Alzheimer’s Disease Using Machine Learning Classification of Multicenter DTI Data,” *PLoS One*, vol. 8, no. 5, p. 64925, 2013.
- [83] R. B. Patil, R. Piyush, and S. Ramakrishnan, “Identification of brain white matter regions for diagnosis of Alzheimer using Diffusion Tensor Imaging,” in *Proceedings of the Annual International Conference of the IEEE Engineering in Medicine and Biology Society, EMBS*, 2013, pp. 6535–6538.
- [84] S. Haller *et al.*, “Individual classification of mild cognitive impairment subtypes by support vector machine analysis of white matter DTI,” *Am. J. Neuroradiol.*, vol. 34, no. 2, pp. 283–291, 2013.
- [85] W. Lee, B. Park, and K. Han, “Classification of diffusion tensor images for the early detection of Alzheimer’s disease,” *Comput. Biol. Med.*, vol. 43, no. 10, pp. 1313–1320, 2013.
- [86] C.-Y. Wee *et al.*, “Identification of MCI individuals using structural and functional connectivity networks,”

- Neuroimage*, vol. 59, no. 3, pp. 2045–56, Feb. 2012.
- [87] L. O'Dwyer *et al.*, "Using support vector machines with multiple indices of diffusion for automated classification of mild cognitive impairment," *PLoS One*, vol. 7, no. 2, p. 32441, 2012.
  - [88] L. O'Dwyer *et al.*, "White matter differences between healthy young ApoE4 carriers and non-carriers identified with tractography and support vector machines," *PLoS One*, vol. 7, no. 4, p. e36024, Apr. 2012.
  - [89] C.-Y. Wee *et al.*, "Neonatal neural networks predict children behavioral profiles later in life," *Hum. Brain Mapp.*, vol. 38, no. 3, pp. 1362–1373, Mar. 2017.
  - [90] D. S. Tylee *et al.*, "Machine-learning classification of 22q11.2 deletion syndrome: A diffusion tensor imaging study," *NeuroImage Clin.*, vol. 15, pp. 832–842, 2017.
  - [91] M. L. Krishnan *et al.*, "Machine learning shows association between genetic variability in PPARG and cerebral connectivity in preterm infants," *Proc. Natl. Acad. Sci. U. S. A.*, vol. 114, no. 52, pp. 13744–13749, Dec. 2017.
  - [92] Z. Cui, Z. Xia, M. Su, H. Shu, and G. Gong, "Disrupted white matter connectivity underlying developmental dyslexia: A machine learning approach," *Hum. Brain Mapp.*, vol. 37, no. 4, pp. 1443–1458, 2016.
  - [93] Y. G. Chimento, B. G. Zaporain, I. S. Prieto, and B. Fernandez-Ruano, "Automatic classification of dyslexic children by applying machine learning to fMRI images," in *Bio-Medical Materials and Engineering*, 2014, vol. 24, no. 6, pp. 2995–3002.
  - [94] H. Lei *et al.*, "Parkinson's Disease Diagnosis via Joint Learning from Multiple Modalities and Relations," *IEEE J. Biomed. Heal. Informatics*, vol. 23, no. 4, pp. 1437–1449, 2019.
  - [95] L. Jin, Q. Zeng, J. He, Y. Feng, S. Zhou, and Y. Wu, "A ReliefF-SVM-based method for marking dopamine-based disease characteristics: A study on SWEDD and Parkinson's disease," *Behav. Brain Res.*, vol. 356, pp. 400–407, Jan. 2019.
  - [96] R. Morisi *et al.*, "Multi-class parkinsonian disorders classification with quantitative MR markers and graph-based features using support vector machines," *Park. Relat. Disord.*, vol. 47, pp. 64–70, 2018.
  - [97] G. Du *et al.*, "Combined diffusion tensor imaging and apparent transverse relaxation rate differentiate Parkinson disease and atypical parkinsonism," *Am. J. Neuroradiol.*, vol. 38, no. 5, pp. 966–972, May 2017.
  - [98] Y. Liu, Y. Wang, C. Huang, and D. Zeng, "Estimating personalized diagnostic rules depending on individualized characteristics," *Stat. Med.*, vol. 36, no. 7, pp. 1099–1117, Mar. 2017.
  - [99] H. Liu *et al.*, "Folded concave penalized learning in identifying multimodal MRI marker for Parkinson's disease," *J. Neurosci. Methods*, vol. 268, pp. 1–6, 2016.
  - [100] A. Cherubini *et al.*, "Magnetic resonance support vector machine discriminates between Parkinson disease and progressive supranuclear palsy," *Mov. Disord.*, vol. 29, no. 2, pp. 266–269, 2014.
  - [101] A. Cherubini *et al.*, "Magnetic resonance support vector machine discriminates essential tremor with rest tremor from tremor-dominant Parkinson disease," *Mov. Disord.*, vol. 29, no. 9, pp. 1216–1219, 2014.
  - [102] S. Haller, S. Badoud, D. Nguyen, V. Garibotto, K. O. Lovblad, and P. R. Burkhard, "Individual detection of patients with Parkinson Disease using support vector machine analysis of diffusion tensor imaging data: Initial results," *Am. J. Neuroradiol.*, vol. 33, no. 11, pp. 2123–2128, Dec. 2012.
  - [103] B. C. Munsell *et al.*, "Relationship between neuronal network architecture and naming performance in temporal lobe epilepsy: A connectome based approach using machine learning," *Brain and Language*, vol. 193. Academic Press Inc., pp. 45–57, Jun-2019.
  - [104] C. hyun Park and S. H. Ohn, "A challenge of predicting seizure frequency in temporal lobe epilepsy using neuroanatomical features," *Neurosci. Lett.*, vol. 692, pp. 115–121, 2019.
  - [105] E. Moulton, R. Valabregue, S. Lehericy, Y. Samson, and C. Rosso, "Multivariate prediction of functional outcome using lesion topography characterized by acute diffusion tensor imaging," *NeuroImage Clin.*, vol. 23, p. 101821, Jan. 2019.
  - [106] K. Mithani *et al.*, "Connectomic Profiling Identifies Responders to Vagus Nerve Stimulation," *Ann. Neurol.*, vol. 86, no. 5, pp. 743–753, Nov. 2019.
  - [107] S. Payabvash *et al.*, "Diffusion tensor tractography in children with sensory processing disorder: Potentials for devising machine learning classifiers," *NeuroImage Clin.*, vol. 23, Jan. 2019.
  - [108] E. Gleichgerricht *et al.*, "Deep learning applied to whole-brain connectome to determine seizure control after epilepsy surgery," *Epilepsia*, vol. 59, no. 9, pp. 1643–1654, Sep. 2018.
  - [109] M. Zurita *et al.*, "Characterization of relapsing-remitting multiple sclerosis patients using support vector machine classifications of functional and diffusion MRI data," *NeuroImage Clin.*, vol. 20, no. September, pp. 724–730, 2018.
  - [110] P. N. Taylor *et al.*, "The impact of epilepsy surgery on the structural connectome and its relation to outcome," *NeuroImage Clin.*, vol. 18, pp. 202–214, 2018.
  - [111] Y. Wang *et al.*, "Voxel-based automated detection of focal cortical dysplasia lesions using diffusion tensor imaging and T2-weighted MRI data," *Epilepsy Behav.*, vol. 84, pp. 127–134, 2018.
  - [112] A. Sarica *et al.*, "The corticospinal tract profile in amyotrophic lateral sclerosis," *Hum. Brain Mapp.*, vol. 38, no. 2, pp. 727–739, 2017.
  - [113] H. Wen *et al.*, "Disrupted topological organization of structural networks revealed by probabilistic diffusion tractography in Tourette syndrome children," *Hum. Brain Mapp.*, vol. 38, no. 8, pp. 3988–4008, Aug. 2017.
  - [114] J. Del Gaizo *et al.*, "Using machine learning to classify temporal lobe epilepsy based on diffusion MRI," *Brain Behav.*, vol. 7, no. 10, 2017.
  - [115] J. Underwood *et al.*, "Gray and White Matter Abnormalities in Treated Human Immunodeficiency Virus Disease and

- Their Relationship to Cognitive Function,” *Clin. Infect. Dis.*, vol. 65, no. 3, pp. 422–432, 2017.
- [116] P. Fang, J. An, L. L. Zeng, H. Shen, S. Qiu, and D. Hu, “Mapping the convergent temporal epileptic network in left and right temporal lobe epilepsy,” *Neurosci. Lett.*, vol. 639, pp. 179–184, 2017.
  - [117] P. M. Ferraro *et al.*, “Multimodal structural MRI in the diagnosis of motor neuron diseases,” *NeuroImage Clin.*, vol. 16, pp. 240–247, 2017.
  - [118] Y. Garcia-Chimeno, B. Garcia-Zapirain, M. Gomez-Beldarrain, B. Fernandez-Ruanova, and J. C. Garcia-Monco, “Automatic migraine classification via feature selection committee and machine learning techniques over imaging and questionnaire data,” *BMC Med. Inform. Decis. Mak.*, vol. 17, no. 1, p. 38, Apr. 2017.
  - [119] K. Kamiya *et al.*, “Machine learning of dti structural brain connectomes for lateralization of temporal lobe epilepsy,” *Magn. Reson. Med. Sci.*, vol. 15, no. 1, pp. 121–129, 2016.
  - [120] H. J. Chen, R. Chen, M. Yang, G. J. Teng, and E. H. Herskovits, “Identification of minimal hepatic encephalopathy in patients with cirrhosis based on white matter imaging and Bayesian data mining,” *Am. J. Neuroradiol.*, vol. 36, no. 3, pp. 481–487, 2015.
  - [121] B. C. Munsell *et al.*, “Evaluation of machine learning algorithms for treatment outcome prediction in patients with epilepsy based on structural connectome data,” *Neuroimage*, vol. 118, pp. 219–230, Sep. 2015.
  - [122] D. Pustina *et al.*, “Predicting the laterality of temporal lobe epilepsy from PET, MRI, and DTI: A multimodal study: Predicting temporal lobe epilepsy laterality,” *NeuroImage Clin.*, vol. 9, pp. 20–31, 2015.
  - [123] D. Cantor-Rivera, A. R. Khan, M. Goubiran, S. M. Mirsattari, and T. M. Peters, “Detection of temporal lobe epilepsy using support vector machines in multi-parametric quantitative MR imaging,” *Comput. Med. Imaging Graph.*, vol. 41, pp. 14–28, 2015.
  - [124] I. Amarreh, M. E. Meyerand, C. Stafstrom, B. P. Hermann, and R. M. Birn, “Individual classification of children with epilepsy using support vector machine with multiple indices of diffusion tensor imaging,” *NeuroImage Clin.*, vol. 4, pp. 757–764, 2014.
  - [125] J. An, P. Fang, W. Wang, Z. Liu, D. Hu, and S. Qiu, “Decreased white matter integrity in mesial temporal lobe epilepsy: A machine learning approach,” *Neuroreport*, vol. 25, no. 10, pp. 788–794, 2014.
  - [126] J. V. Stough, J. Glaister, C. Ye, S. H. Ying, J. L. Prince, and A. Carass, “Automatic method for thalamus parcellation using multi-modal feature classification,” in *Lecture Notes in Computer Science (including subseries Lecture Notes in Artificial Intelligence and Lecture Notes in Bioinformatics)*, 2014, vol. 8675 LNCS, no. PART 3, pp. 169–176.
  - [127] M. J. Paldino, K. Hedges, and W. Zhang, “Independent contribution of individual white matter pathways to language function in pediatric epilepsy patients,” *NeuroImage Clin.*, vol. 6, pp. 327–332, 2014.
  - [128] E. Ziv, O. Tymofiyeva, D. M. Ferriero, A. J. Barkovich, C. P. Hess, and D. Xu, “A machine learning approach to automated structural network analysis: Application to neonatal encephalopathy,” *PLoS One*, vol. 8, no. 11, 2013.
  - [129] N. K. Focke, M. Yogarajah, M. R. Symms, O. Gruber, W. Paulus, and J. S. Duncan, “Automated MR image classification in temporal lobe epilepsy,” *Neuroimage*, vol. 59, no. 1, pp. 356–362, 2012.
  - [130] L. G. Goetschius *et al.*, “Amygdala-prefrontal cortex white matter tracts are widespread, variable and implicated in amygdala modulation in adolescents,” *Neuroimage*, vol. 191, pp. 278–291, 2019.
  - [131] Y. Mu, Q. Li, and Y. Zhang, “White Matter Segmentation Algorithm for DTI Images Based on Super-Pixel Full Convolutional Network,” *J. Med. Syst.*, vol. 43, no. 9, 2019.
  - [132] F. Deng *et al.*, “Plasticity in deep and superficial white matter: a DTI study in world class gymnasts,” *Brain Struct. Funct.*, vol. 223, no. 4, pp. 1849–1862, 2018.
  - [133] L. Li *et al.*, “Abnormal brain structure as a potential biomarker for venous erectile dysfunction: evidence from multimodal MRI and machine learning,” *Eur. Radiol.*, vol. 28, no. 9, pp. 3789–3800, 2018.
  - [134] S. H. Park *et al.*, “Alcohol use effects on adolescent brain development revealed by simultaneously removing confounding factors, identifying morphometric patterns, and classifying individuals,” *Sci. Rep.*, vol. 8, no. 1, pp. 1–14, Dec. 2018.
  - [135] Y. Wen and L. He, “A statistical approach to segmentation of diffusion tensor imaging,” in *Bio-Medical Materials and Engineering*, 2014, vol. 24, no. 1, pp. 1253–1259.
  - [136] X. Hao and P. T. Fletcher, “Joint fractional segmentation and multi-tensor estimation in diffusion MRI,” in *Lecture Notes in Computer Science (including subseries Lecture Notes in Artificial Intelligence and Lecture Notes in Bioinformatics)*, 2013, vol. 7917 LNCS, pp. 340–351.
  - [137] E. Aliotta, H. Nourzadeh, J. Sanders, D. Muller, and D. B. Ennis, “Highly accelerated, model-free diffusion tensor MRI reconstruction using neural networks,” *Med. Phys.*, vol. 46, no. 4, pp. 1581–1591, Apr. 2019.
  - [138] T. Kuhn *et al.*, “An augmented aging process in brain white matter in HIV,” *Hum. Brain Mapp.*, vol. 39, no. 6, pp. 2532–2540, 2018.
  - [139] G. Ball, R. Beare, and M. L. Seal, “Network component analysis reveals developmental trajectories of structural connectivity and specific alterations in autism spectrum disorder,” *Hum. Brain Mapp.*, vol. 38, no. 8, pp. 4169–4184, Aug. 2017.
  - [140] J. D. Medaglia *et al.*, “Brain network efficiency is influenced by the pathologic source of corticobasal syndrome,” *Neurology*, vol. 89, no. 13, pp. 1373–1381, Sep. 2017.
  - [141] A. Besga *et al.*, “Eigenanatomy on Fractional Anisotropy Imaging Provides White Matter Anatomical Features Discriminating Between Alzheimer’s Disease and Late Onset Bipolar Disorder,” *Curr. Alzheimer Res.*, vol. 13, no. 5, pp. 557–565, 2016.

- [142] A. Yendiki, M. Reuter, P. Wilkens, H. D. Rosas, and B. Fischl, "Joint reconstruction of white-matter pathways from longitudinal diffusion MRI data with anatomical priors," *Neuroimage*, vol. 127, pp. 277–286, Feb. 2016.
- [143] C. J. Lin *et al.*, "Connectivity features for identifying cognitive impairment in presymptomatic carotid stenosis," *PLoS One*, vol. 9, no. 1, p. e85441, 2014.
- [144] N. Adluru, B. M. Hanlon, A. Lutz, J. E. Lainhart, A. L. Alexander, and R. J. Davidson, "Penalized likelihood phenotyping: Unifying voxelwise analyses and multi-voxel pattern analyses in neuroimaging," *Neuroinformatics*, vol. 11, no. 2, pp. 227–247, 2013.
- [145] C. Y. Chu, J. P. Huang, C. Y. Sun, Y. L. Zhang, W. Y. Liu, and Y. M. Zhu, "Multifiber pathway reconstruction using bundle constrained streamline," *Comput. Med. Imaging Graph.*, vol. 46, pp. 291–299, Dec. 2015.
- [146] T. Zhang *et al.*, "Predicting cortical ROIs via joint modeling of anatomical and connectional profiles," *Med. Image Anal.*, vol. 17, no. 6, pp. 601–615, Aug. 2013.
- [147] Y. Ghanbari, J. Herrington, R. C. Gur, R. T. Schultz, and R. Verma, "Locality preserving non-negative basis learning with graph embedding," in *Lecture Notes in Computer Science (including subseries Lecture Notes in Artificial Intelligence and Lecture Notes in Bioinformatics)*, 2013, vol. 7917 LNCS, pp. 316–327.
- [148] A. Besga, M. Termenon, M. Graña, J. Echeveste, J. M. Pérez, and A. Gonzalez-Pinto, "Discovering Alzheimer's disease and bipolar disorder white matter effects building computer aided diagnostic systems on brain diffusion tensor imaging features," *Neurosci. Lett.*, vol. 520, no. 1, pp. 71–76, Jun. 2012.
